# Supplementary material for: Neutron drip line in the Ca region from Bayesian model averaging
Source: arXiv:1901.07632 ancillary file (2020-01-16)
Supplement: Supplementary file 1 [file Ca-Bayes-PRL-supp.pdf]

# Supplemental Material for "Neutron drip line in the Ca region from Bayesian model averaging"

Léo Neufcourt,[1,2] Yuchen Cao (曹宇晨),[3] Witold Nazarewicz,[4] Erik Olsen,[2] and Frederi Viens[1]

[1]*Department of Statistics and Probability, Michigan State University, East Lansing, Michigan 48824, USA*
[2]*FRIB Laboratory, Michigan State University, East Lansing, Michigan 48824, USA*
[3]*Department of Physics and Astronomy and NSCL Laboratory, Michigan State University, East Lansing, Michigan 48824, USA*
[4]*Department of Physics and Astronomy and FRIB Laboratory, Michigan State University, East Lansing, Michigan 48824, USA*

This supplemental material contains additional figures, including figures of extrapolated separation energies for the Ti isotopic chain (I A); posterior probability of existence for different models (I B); plots of empirical coverage probabilities (I C); and a plot of HFB-24 predictions for the calcium chain (I D). Section II contains supplemental discussion of DFT calculations of odd-$A$ and odd-odd nuclei (Sec. II A); description of the Gaussian process model and parameters (Sec. II B) and Gaussian process evaluation (Sec. II C); and discussion of our model averaging procedure (Sec. II D). Finally, supplemental tables are contained in Sec. III. Those include: posterior weights of nuclear mass models (III A); root-mean-square deviations obtained in testing calculations (III B); and posterior probabilities of existence of nuclei from the neutron-rich Ca region (III C).

# I. SUPPLEMENTAL FIGURES

## A. Extrapolated separation energies for the Ti isotopic chain

Figure S1 shows extrapolated separation energies for the Ti isotopic chain for three global mass models corrected with the GP emulator.

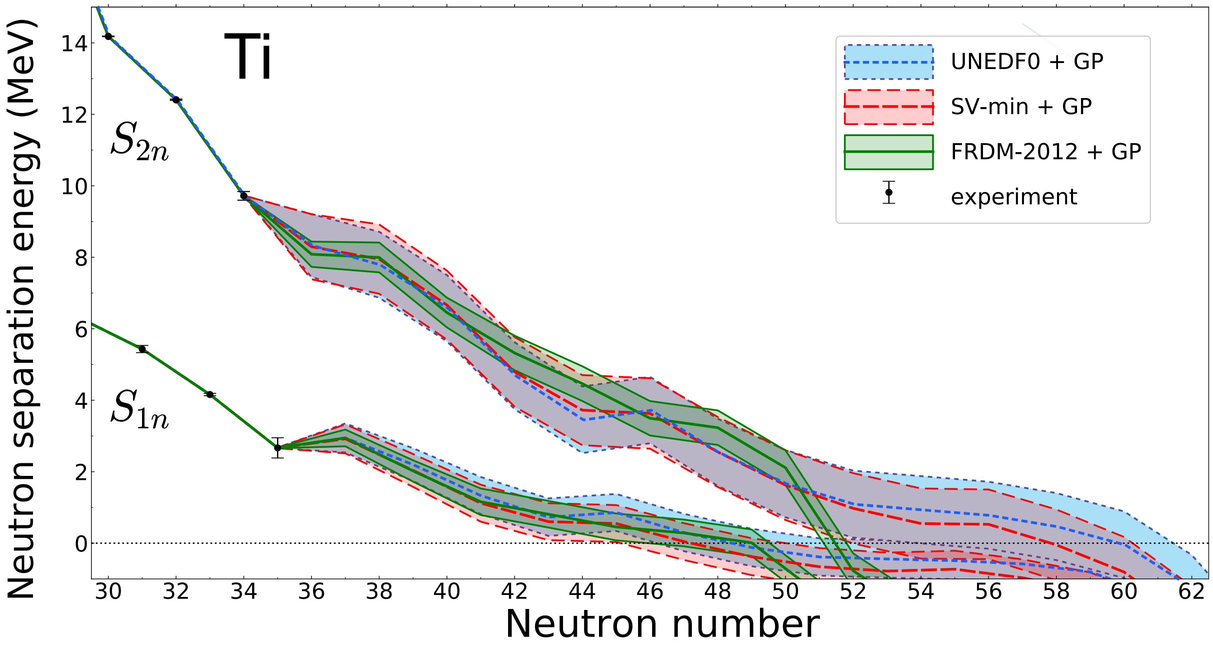


FIG. S1. Extrapolations of $S_{1n}$ and $S_{2n}$ for the Ti chain corrected with GP and one-sigma CIs, combined for three representative models. The solid lines show the average prediction while the shaded bands give one-sigma CIs.

## B. Posterior probability existence for different models

In addition to Fig. 3 we include here results for individual models: SLy4 (Fig. S2), SkP (Fig. S3), SkM* (Fig. S4), SV-min (Fig. S5), UNEDF0 (Fig. S6), UNEDF1 (Fig. S7), UNEDF2 (Fig. S8), FRDM-2012 (Fig. S9), and HFB-24 (Fig. S10). We note that different models can produce diverse ranges for the domain of stable nuclei and predictions for the neutron drip line location. For instance SLy4 predicts the neutron drip line for significantly lighter nuclei than SkM*. HFB-24 predicts holes for the isotones $N = 43$ and 47. Additionally, the observed isotopes $^{49}$S, $^{52}$Cl and $^{53}$Ar are predicted to be neutron-unbound by several models. According to AME2016 extrapolations, $S_{1n}$ of $^{49}$S and $^{53}$Ar are close to zero. We also note that the theoretical error on $S_{1n}$ is around 400 keV for threshold systems; hence, it is not surprising that estimated values of $p_{ex}$ exhibit significant variations across models (see Tables S3-S7).

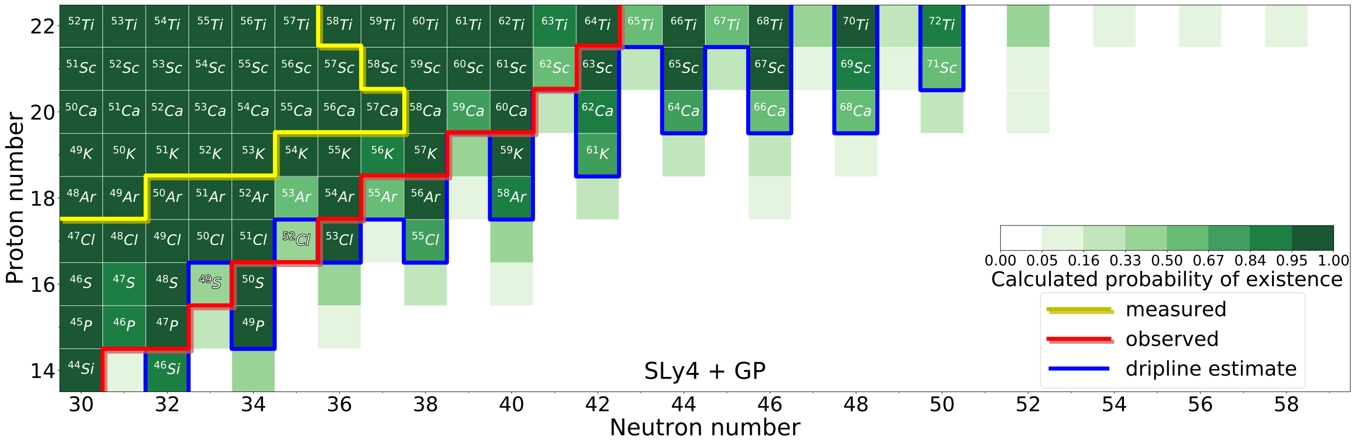


FIG. S2. Similar to Fig. 3 but for SLy4+GP.

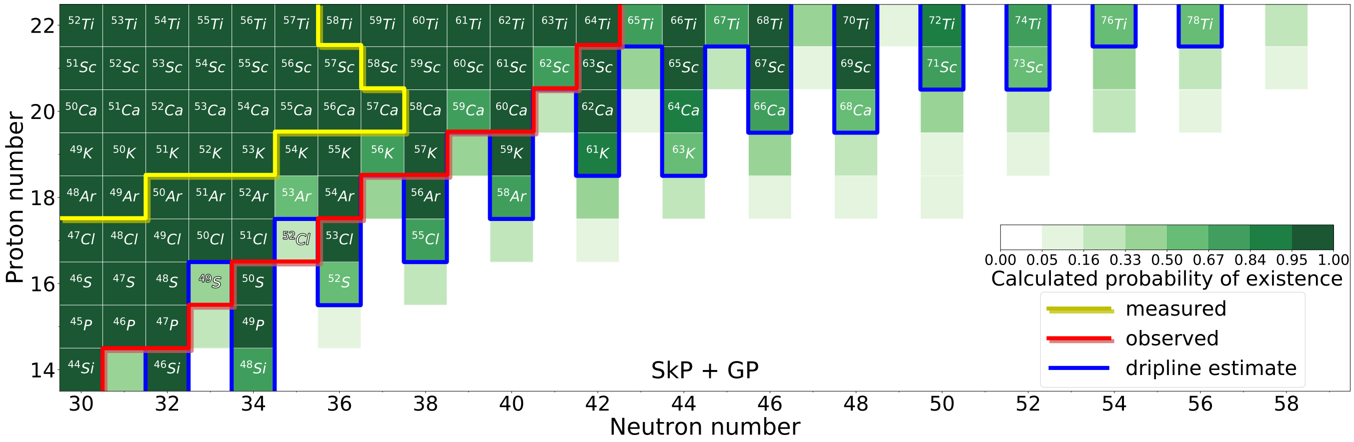


FIG. S3. Similar to Fig. 3 but for SkP+GP.

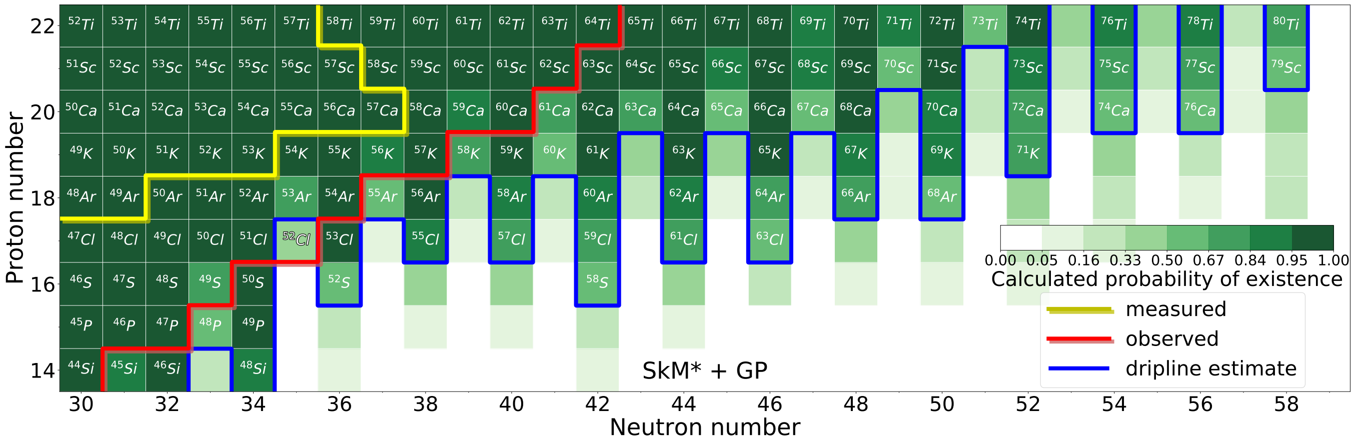


FIG. S4. Similar to Fig. 3 but for SkM*+GP.

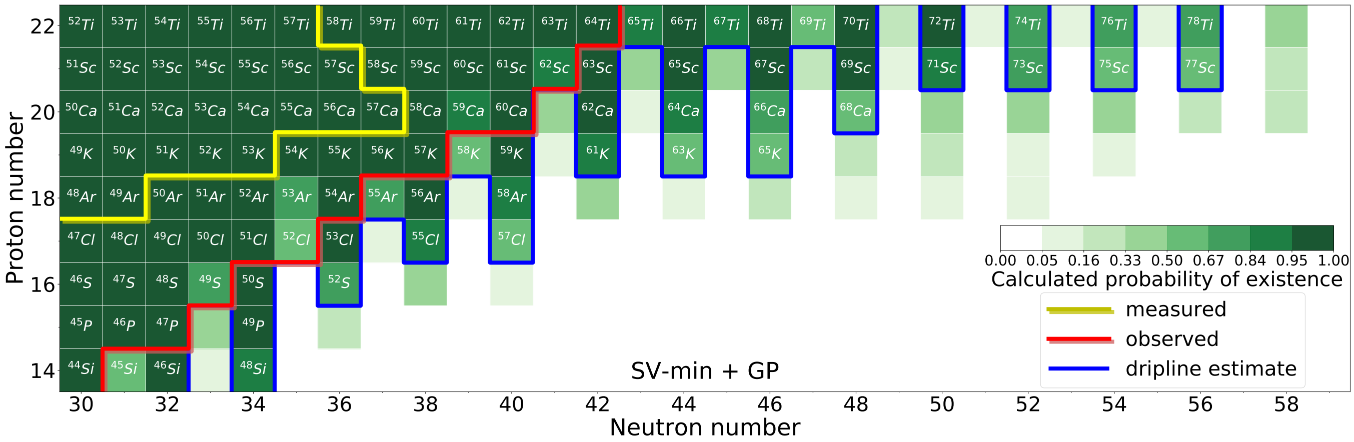


FIG. S5. Similar to Fig. 3 but for SV-min+GP.

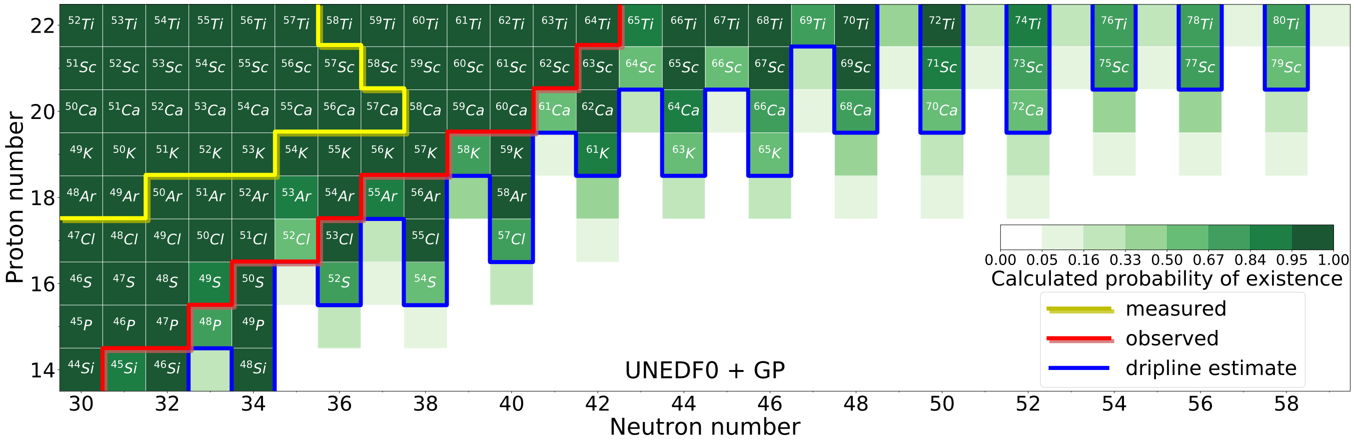


FIG. S6. Similar to Fig. 3 but for UNEDF0+GP.

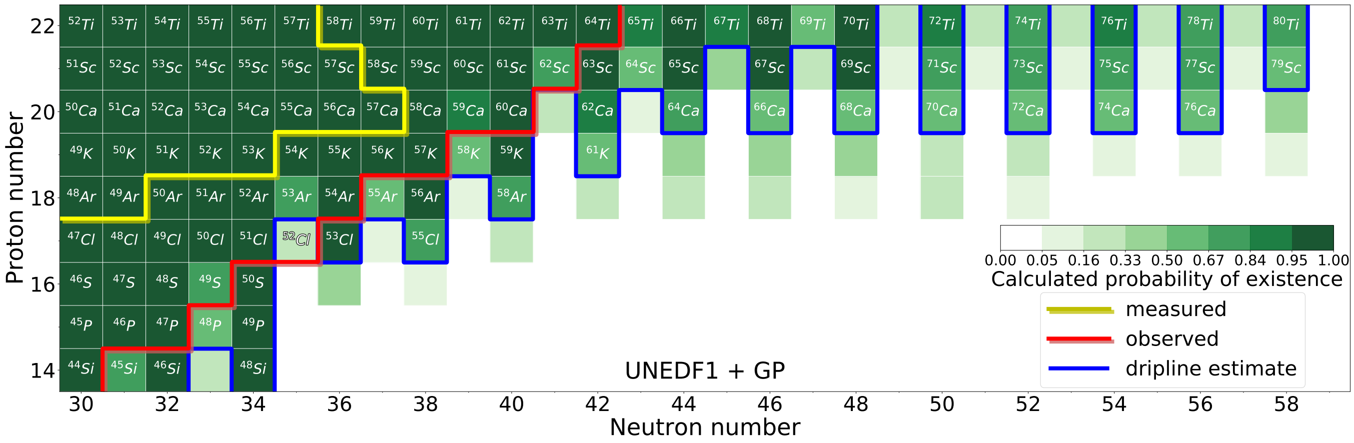


FIG. S7. Similar to Fig. 3 but for UNEDF1+GP.

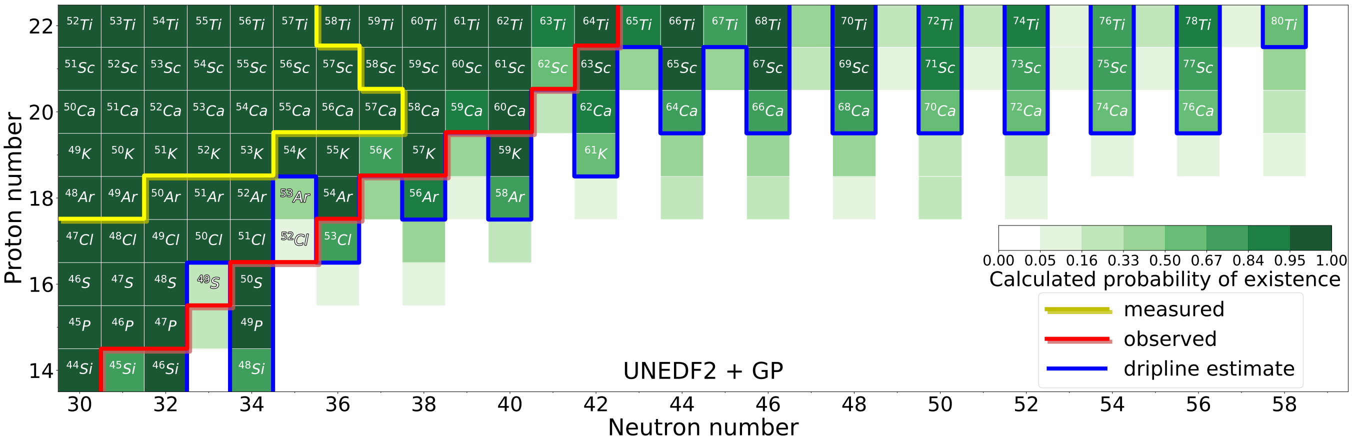


FIG. S8. Similar to Fig. 3 but for UNEDF2+GP.

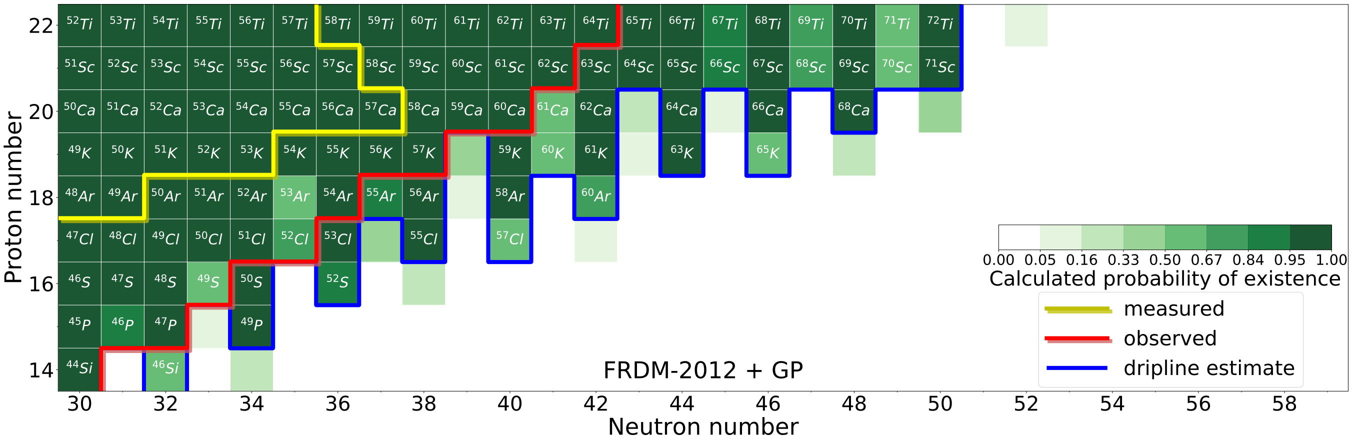


FIG. S9. Similar to Fig. 3 but for FRDM-2012+GP.

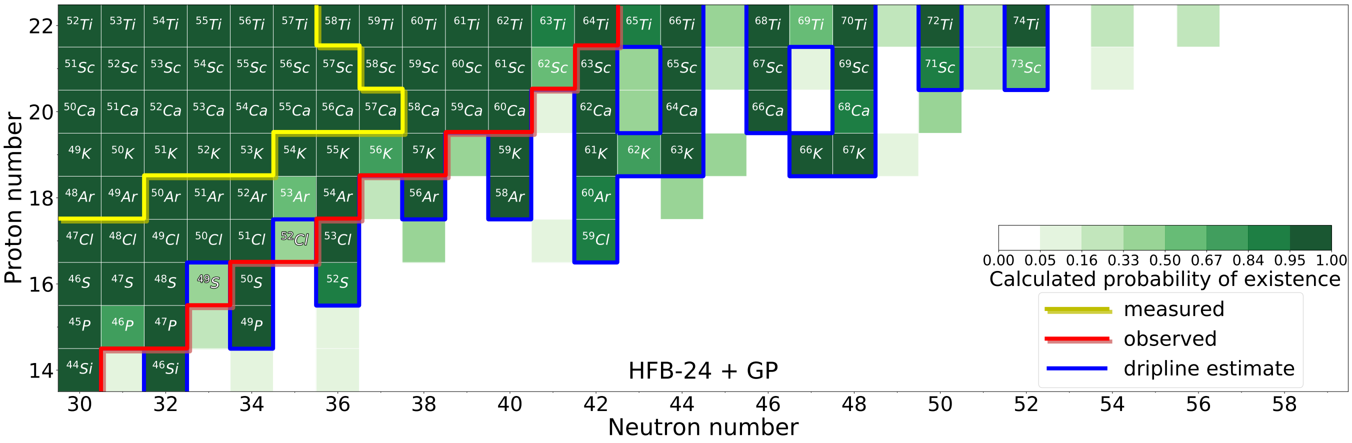


FIG. S10. Similar to Fig. 3 but for HFB-24+GP.

### C. Empirical coverage probabilities

Figure S11 shows what is known as the empirical coverage probability (ECP), which is a simple and intuitive metric for assessing the quality of a statistical model's quantification of uncertainty. The ECP curve corresponds to the proportion of the testing data which actually falls inside the predicted credibility intervals (CIs) as a function of the credibility level. For perfect uncertainty quantification, one would obtain a straight line. We obtain similar curves for all nuclear models, for one- and two-neutron separation energies, and for even-$Z$ and odd-$Z$ chains. The matching of the nominal value is overall satisfactory, with an inflection point at the middle of the curve: our CIs are slightly too optimistic at low credibility levels, and slightly too conservative at (most important) high credibility levels.

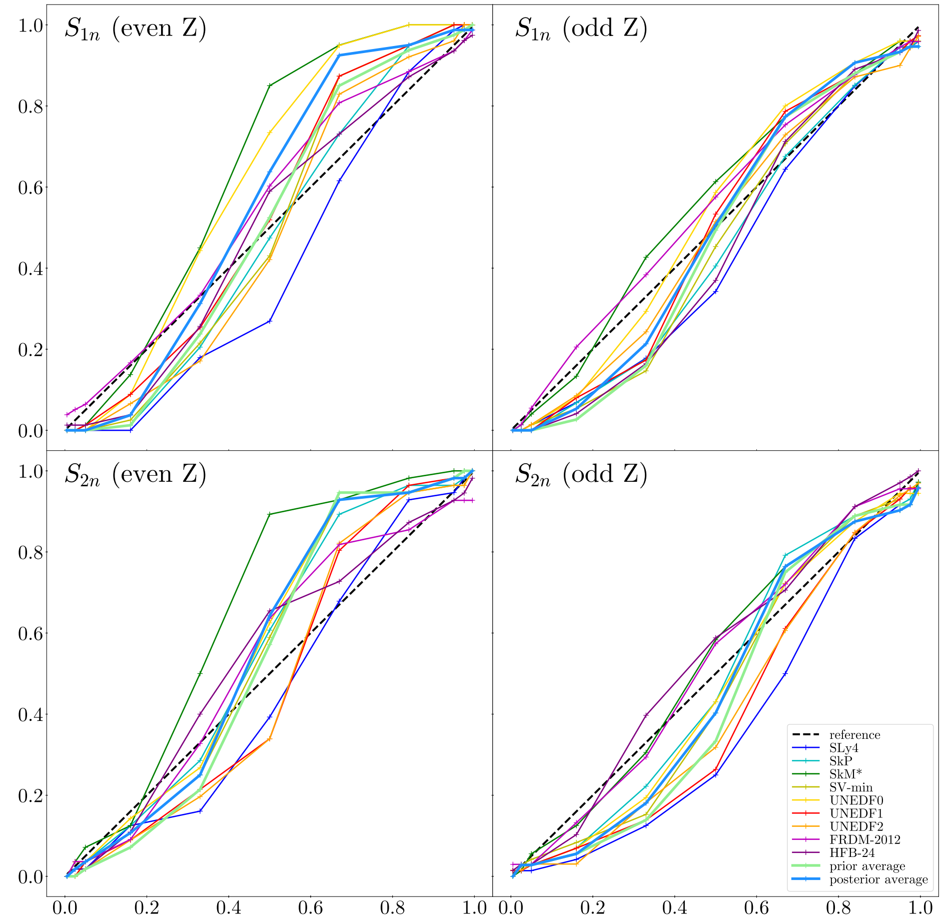


FIG. S11. Empirical coverage probability for all models considered.

### D. HFB-24 predictions for the calcium chain

As seen in Fig. 1, HFB-24 shows a large deviation of $S_{1n}$ for $^{55}$Ca as compared to other models. The values of $S_{1n}$ and $S_{2n}$ for the Ca chain predicted in HFB-24+GP are shown in Fig. S12 with statistical training on AME2003 and AME2016+RIKEN2018. It is seen that the above-mentioned deviation can be traced back to a kink in $S_{1n}$ at $N = 35$. Another kink, but for $S_{2n}$, is also predicted at $N = 44$. Other models displayed in Fig. 2 provide a fairly smooth behavior of separation energies.

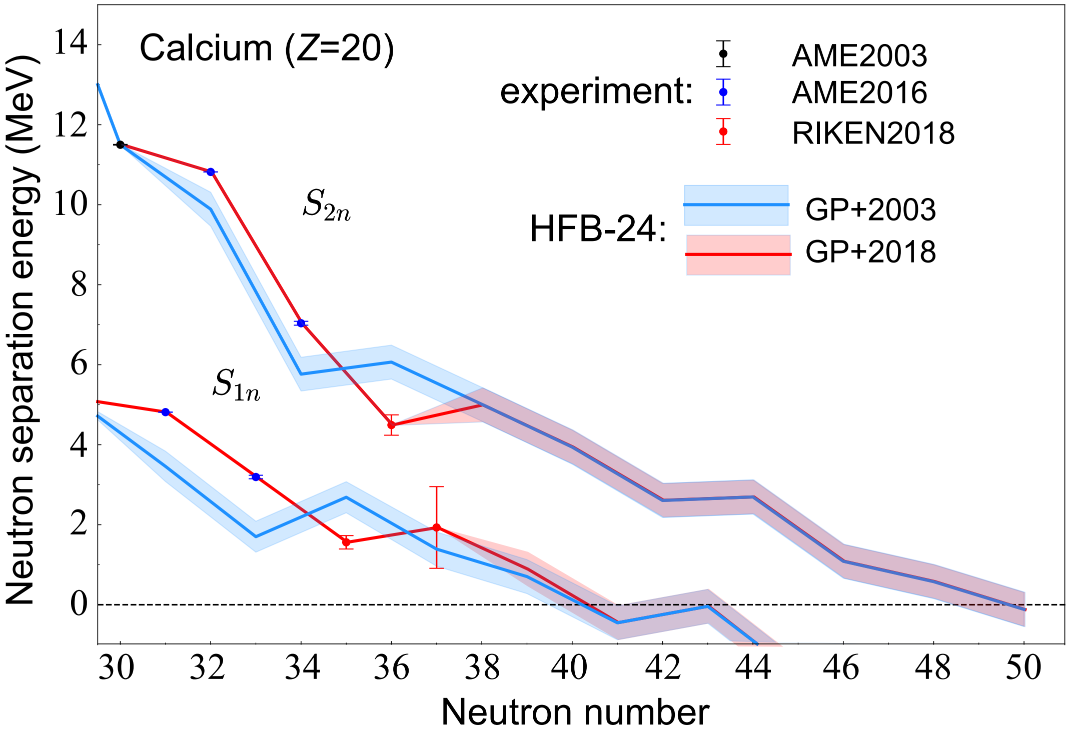


FIG. S12. Extrapolations of $S_{1n}$ and $S_{2n}$ for the Ca isotopic chain obtained in HFB-24 corrected with GP and one-sigma CIs using the AME2003 (GP+2003) and AME2016$^*$+RIKEN2018 (GP+2018) training datasets. The solid lines show the average prediction while the shaded bands give one-sigma CIs.

## II. SUPPLEMENTAL DISCUSSION

### A. DFT calculations of odd-$A$ and odd-odd nuclei

The DFT calculations of nuclear binding energies $B(Z, N)$ were carried out for even-even nuclei as we want to avoid additional complications and uncertainties related to the choice and treatment of quasi-particle configurations in odd-$A$ and odd-odd systems [36]. The neutron separation energies are given by

$$S_{1n}(Z, N) = B(Z, N) - B(Z, N - 1), \tag{3}$$
$$S_{2n}(Z, N) = B(Z, N) - B(Z, N - 2), \tag{4}$$

where we assume that the binding energy is defined with positive sign. To estimate $B(Z, N)$ for nuclei with odd particle numbers, we reduce the average binding energy of two even-$N$, or even-$Z$ neighbors by the mean pairing gap. For instance, for odd neutron number

$$B(Z, N) \approx \frac{1}{2}\left[B(Z, N - 1) + B(Z, N + 1)\right] - \frac{1}{2}\left[\Delta_n(Z, N - 1) + \Delta_n(Z, N + 1)\right], \tag{5}$$

where $\Delta_n(Z, N)$ is the average value of the neutron pairing gap [26].

## B. GP model and parameters

Based on the comparative analysis previously performed recently between GP and BNN on the $S_{2n}$ of even-even nuclei [24], we retained the GP for the statistical (Bayesian likelihood) model

$$y_i = f(x_i, \theta) + \sigma\epsilon_i. \tag{6}$$

A GP is a Gaussian field, i.e., a Gaussian functional on the two-dimensional nuclear domain indexed by $x = (Z, N)$, which is characterized by its mean and covariance [24, 42], for which a parametrization must be selected. We take the mean function to be 0, and in order to model the "spatial" dependence of nearby nuclei in the nuclear landscape, we use an exponential quadratic covariance kernel

$$k_{\eta,\rho}(x, x') := \eta^2 e^{-\frac{(Z-Z')^2}{2\rho_Z^2} - \frac{(N-N')^2}{2\rho_N^2}}, \tag{7}$$

where the parameters $\theta \equiv \{\eta, \rho_Z, \rho_N\}$ have a straightforward interpretation: $\eta$ defines the scale and $\rho_Z$ and $\rho_N$ are characteristic correlation ranges in the proton and neutron direction, respectively. Thus the function $f(x, \theta)$ in 6, which represents the output of the physical model, can be written with here $\theta := (\eta, \rho_Z, \rho_N)$ as

$$f(x, \theta) \sim \mathcal{GP}(0, k_{\eta,\rho}(x, x')). \tag{8}$$

Figure S13 shows the posterior distribution of those three parameters which are bell-shaped. Posterior distributions are more regular for $S_{2n}$ than $S_{1n}$, and more regular for even-$Z$ chains than odd-$Z$ chains. In any case, these three parameters are very well constrained, and the range of variations is very small. An analysis of the histograms (or of the corresponding parameter samples) tells us that roughly 90% of the correlation effects, which are about twice as strong for $S_{2n}$ than for $S_{1n}$, occur within a range of ± two neutrons and three protons for $S_{1n}$ and ± three neutrons and two protons for $S_{2n}$.

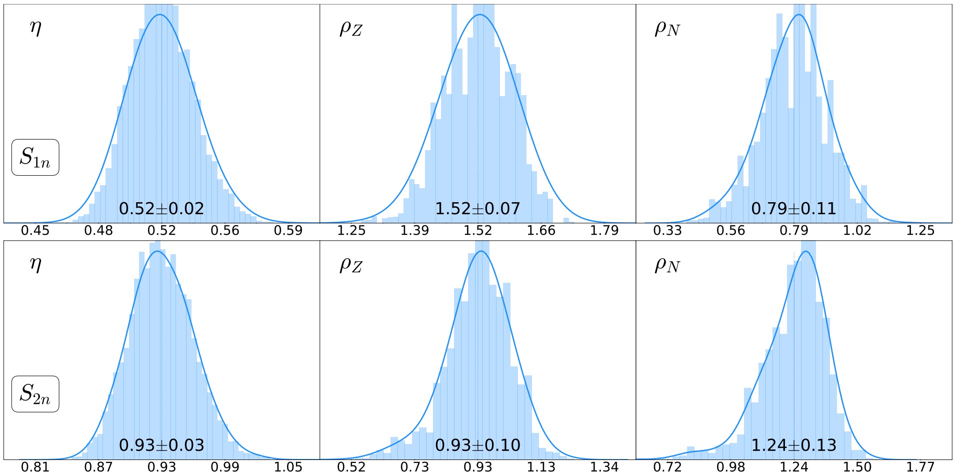


FIG. S13. Posterior distribution of the GP parameters in the UNEDF0 variant of calculations for $S_{1n}$ (top) and $S_{2n}$ (bottom) in even-$Z$ nuclei using the 2018 training dataset. For each parameter $\eta$, $\rho_Z$, $\rho_N$, the solid line smoothens the background histogram, which shows the distribution of the posterior samples; the dashed line gives the posterior average value. Posterior mean and standard deviation are indicated by numbers.

## C. GP evaluation

In our previous work [24] the predictive power of the GP was assessed in comparison to Bayesian Neural Networks (BNN) for the two-neutron separation energies of even-even nuclei on 12 nuclear models. We relied on two criteria, the improvement of the prediction and the *honesty* of the credibility intervals, respectively measured by the improvement of the rms deviation and the empirical coverage probability curve (see Fig.S11) while using a testing set (AME2016-AME2003) at the external boundary of the training set (AME2003). In particular we concluded that the reduction of the rms deviation was decreasing when going from DFT models to more phenomenological models, which all

achieved comparable deviations after statistical correction. In this study, for similar models, we achieve comparable performances on odd-$Z$ nuclei and on one-neutron separation energies, with prediction improvements ranging from 10% to 30% for most models (see Table S2). Similarly as we observed for the $S_{2n}$ of even-even nuclei, all models have similar rms deviations on each observable after the GP correction. Across observables, the GP refinement performs best on $S_{1n}$ data and on odd-$Z$ chains.

It is to be noted that AME2016 contains data on remeasured masses since the AME2003 compilation. In some cases, the differences between old and new data can be significant (up to 30% ), especially for light nuclei. Given the overall consensus that the AME2016 values are more accurate, the points in question are removed from the AME2003 training dataset, similarly as in Ref. [24]. In the case of $S_{2n}$ values of even-even nuclei, this concerns $^{24}$O, $^{34}$Mg and $^{52}$Ca. Of course this correction is applied only to the emulator trained on AME2003, solely for the purpose of calculating meaningful rms deviations, and all other training sets incorporate the most recent measurement available to date.

A meticulous reader will notice variations between the values of the rms deviations of the $S_{2n}$ energies of even-even nuclei provided in Table S2 below and in Table 1 of Ref. [24]. These are due to slightly different choices in data selection: in the present work, theoretical $S_{2n}$ energies for proton-rich nuclei $^{180}$Pb and $^{188}$Po were used for all models while they were ignored in Ref. [24] when the corresponding proton separation energies were negative. Additionally, $^{10}$He, $^{16}$Be, and $^{26}$O for which the experimental $S_{2n}$ values are negative were removed from the testing set AME2016-AME2003 in the present work as they are far from the calcium region, while they were kept in Ref. [24] for completeness.

### D. Model averaging

Given that each mass model corresponds to a subjective optimum for its developers, it is *a priori* difficult to select a best model. We have first presented results regarding an average model where the binding energies are given by the arithmetic average of each model's prediction, followed by a more sophisticated Bayesian average which is a first step towards a fully informed Bayesian model averaging.

Although the naïve average is elementary, we can see that it performs well with respect to rms reduction and matching of the empirical coverage probabilities. From a Bayesian perspective the complete solution to the averaging problem is formal Bayesian model averaging [56, 57], where this simple average should be reweighted using the model posterior probabilities computed by integrating the respective likelihoods over the parameter space. Applying such an approach is computationally intensive in our framework, and is the object of ongoing research. In the absence of additional information and costly posterior computations, the choice of uniform weights is essentially optimal [58].

We also propose an alternative model averaging based on the knowledge that the nuclei $^{49}$S, $^{52}$Cl and $^{53}$Ar have been recently observed [1, 7]. Our method, which remains in the Bayesian paradigm, is to inform the uniform prior probabilities on the models with the observation data using the likelihood of existence of those three nuclei. Bayes' formula leads us to the computation of the corresponding weights $w_k$ as

$$w_k := p\Big(\mathcal{M}_k|^{52}\mathrm{Cl}, {}^{53}\mathrm{Ar}, {}^{49}\mathrm{S}\ \mathrm{exist}\Big) \propto p\left(S_{1n}(^{49}\mathrm{S}) > 0, S_{1n}(^{52}\mathrm{Cl}) > 0, S_{1n}(^{53}\mathrm{Ar}) > 0|\mathcal{M}_k\right)\pi(\mathcal{M}_k), \tag{9}$$

where $\pi(\mathcal{M}_k)$ are uniform prior weights on each of the nine nuclear models. Thus these weights are all equal to 1/9 and cancel out in the computation of $w_k$. The computed values are listed in Table S1. We emphasize that conditioning with respect to $^{49}$S, $^{52}$Cl and $^{53}$Ar is equivalent to conditioning over the observed nuclei in the whole Ca region, since other experimentally-observed isotopes are predicted to be bound by the global models considered.

## III. SUPPLEMENTAL TABLES

### A. Posterior weights of nuclear mass models

Table S1 lists the posterior weights of each model defined by Eq. (1) corresponding to the training datasets AME2003 and AME2016+RIKEN2018 (used in Fig. 3).

| training set | SLy4 | SkP | SkM* | SV-min | UNEDF0 | UNEDF1 | UNEDF2 | FRDM-2012 | HFB-24 |
|---|---|---|---|---|---|---|---|---|---|
| 2003 | 0.02 | 0.04 | 0.09 | 0.14 | 0.36 | 0.09 | 0.00 | 0.16 | 0.09 |
| 2018 | 0.04 | 0.05 | 0.12 | 0.15 | 0.27 | 0.10 | 0.07 | 0.15 | 0.05 |

TABLE S1. Posterior weights of nuclear physics models obtained by training the GP with the AME2003 and AME2016+RIKEN2018 datasets.

### B. Root-mean-square deviations obtained in testing calculations

Table S2 displays the rms values of $S_{1n}$ and $S_{2n}$ residuals for the testing AME2016-AME2003 dataset, calculated in various mass models with and without the statistical GP treatment of residuals with emulators $\delta^{\rm em}$ trained on the AME2003 dataset. It is seen that the GP reduces the rms residuals noticeably. Overall, for the testing dataset, the rms deviation from experimental $S_{1n}$ and $S_{2n}$ values is around 500 keV for all theoretical models employed in this study, which suggests that our statistical methods capture most of the residual structure. As observed in Ref.[24], whereas there are significant variations in the rms deviations obtained in different models prior to statistical treatment, the differences mostly disappear after the GP refinement.

Additionally, both the naïve and the more involved averaged models achieve the best rms performance overall across all models, both before and after refinement, and a systematically lower rms error than any of the DFT models. This is a clear indication in favor of model averaging, and this provides a call for developing a full-scale model averaging methodology.

| Mass model | $\delta_{1n,\rm rms}$ | | | | $\delta_{2n,\rm rms}$ | | | |
|---|---|---|---|---|---|---|---|---|
| | $Z$-even | | $Z$-odd | | $Z$-even | | $Z$-odd | |
| | raw | GP | raw | GP | raw | GP | raw | GP |
| SLy4 | 0.54 | 0.38 | 0.78 | 0.48 | 0.91 | 0.88 | 0.95 | 0.64 |
| SkP | 0.38 | 0.28 | 0.70 | 0.43 | 0.78 | 0.75 | 0.89 | 0.55 |
| SkM* | 0.64 | 0.40 | 0.70 | 0.46 | 1.22 | 1.01 | 1.23 | 0.61 |
| SV-min | 0.36 | 0.26 | 0.65 | 0.42 | 0.71 | 0.71 | 0.81 | 0.49 |
| UNEDF0 | 0.41 | 0.30 | 0.55 | 0.40 | 0.72 | 0.74 | 0.79 | 0.51 |
| UNEDF1 | 0.37 | 0.30 | 0.50 | 0.36 | 0.64 | 0.64 | 0.74 | 0.48 |
| UNEDF2 | 0.47 | 0.34 | 0.65 | 0.43 | 0.81 | 0.71 | 0.84 | 0.52 |
| FRDM-2012 | 0.45 | 0.34 | 0.38 | 0.33 | 0.60 | 0.56 | 0.49 | 0.39 |
| HFB-24 | 0.47 | 0.38 | 0.46 | 0.35 | 0.40 | 0.40 | 0.42 | 0.40 |
| prior average | 0.33 | 0.25 | 0.54 | 0.37 | 0.57 | 0.56 | 0.61 | 0.44 |
| posterior average | 0.33 | 0.25 | 0.51 | 0.37 | 0.59 | 0.59 | 0.64 | 0.43 |

TABLE S2. Root mean square values of $\delta_{1n}$ and $\delta_{2n}$ (in MeV) for various nuclear models before (raw) and after the GP refinement using the testing AME2016-AME2003 dataset. The training AME2003 dataset was used to compute the emulators $\delta^{\rm stat}$.

### C. Posterior probabilities of existence of nuclei

Tables S3-S7 display calculated $p_{ex}$ values for nuclei from the neutron-rich Ca region.

| N | posterior average | prior average | SLy4 | SkP | SkM* | SV-min | UNEDF0 | UNEDF1 | UNEDF2 | FRDM-2012 | HFB-24 |
|---|---|---|---|---|---|---|---|---|---|---|---|
| 30 | 1.00 | 1.00 | 1.00 | 1.00 | 1.00 | 1.00 | 1.00 | 1.00 | 1.00 | 1.00 | 1.00 |
| 31 | 1.00 | 1.00 | 1.00 | 1.00 | 1.00 | 1.00 | 1.00 | 1.00 | 1.00 | 1.00 | 1.00 |
| 32 | 1.00 | 1.00 | 1.00 | 1.00 | 1.00 | 1.00 | 1.00 | 1.00 | 1.00 | 1.00 | 1.00 |
| 33 | 1.00 | 1.00 | 1.00 | 1.00 | 1.00 | 1.00 | 1.00 | 1.00 | 1.00 | 1.00 | 1.00 |
| 34 | 1.00 | 1.00 | 1.00 | 1.00 | 1.00 | 1.00 | 1.00 | 1.00 | 1.00 | 1.00 | 1.00 |
| 35 | 1.00 | 1.00 | 1.00 | 1.00 | 1.00 | 1.00 | 1.00 | 1.00 | 1.00 | 1.00 | 1.00 |
| 36 | 1.00 | 1.00 | 1.00 | 1.00 | 1.00 | 1.00 | 1.00 | 1.00 | 1.00 | 1.00 | 1.00 |
| 37 | 1.00 | 1.00 | 1.00 | 1.00 | 1.00 | 1.00 | 1.00 | 1.00 | 1.00 | 1.00 | 1.00 |
| 38 | 1.00 | 1.00 | 1.00 | 1.00 | 1.00 | 1.00 | 1.00 | 1.00 | 1.00 | 1.00 | 1.00 |
| 39 | 0.94 | 0.92 | 0.81 | 0.84 | 0.95 | 0.93 | 0.98 | 0.93 | 0.86 | 1.00 | 0.98 |
| 40 | 1.00 | 1.00 | 1.00 | 1.00 | 1.00 | 1.00 | 1.00 | 1.00 | 1.00 | 1.00 | 1.00 |
| 41 | 0.46 | 0.37 | 0.18 | 0.30 | 0.84 | 0.36 | 0.55 | 0.25 | 0.16 | 0.56 | 0.15 |
| 42 | 0.98 | 0.98 | 0.94 | 0.99 | 1.00 | 0.99 | 0.99 | 0.95 | 0.93 | 1.00 | 1.00 |
| 43 | 0.21 | 0.20 | 0.04 | 0.06 | 0.74 | 0.09 | 0.19 | 0.06 | 0.04 | 0.16 | 0.47 |
| 44 | 0.88 | 0.87 | 0.69 | 0.92 | 1.00 | 0.87 | 0.88 | 0.72 | 0.71 | 1.00 | 1.00 |
| 45 | 0.13 | 0.11 | 0.03 | 0.01 | 0.66 | 0.04 | 0.09 | 0.04 | 0.04 | 0.07 | 0.00 |
| 46 | 0.82 | 0.81 | 0.62 | 0.76 | 0.99 | 0.77 | 0.76 | 0.63 | 0.75 | 1.00 | 0.99 |
| 47 | 0.10 | 0.09 | 0.02 | 0.00 | 0.58 | 0.02 | 0.08 | 0.03 | 0.03 | 0.03 | 0.00 |
| 48 | 0.76 | 0.73 | 0.51 | 0.58 | 0.99 | 0.64 | 0.72 | 0.62 | 0.69 | 0.96 | 0.92 |
| 49 | 0.06 | 0.05 | 0.00 | 0.00 | 0.35 | 0.01 | 0.04 | 0.02 | 0.02 | 0.00 | 0.00 |
| 50 | 0.57 | 0.53 | 0.25 | 0.42 | 0.94 | 0.49 | 0.60 | 0.55 | 0.61 | 0.48 | 0.39 |
| 51 | 0.04 | 0.03 | 0.00 | 0.00 | 0.20 | 0.01 | 0.04 | 0.03 | 0.03 | 0.00 | 0.00 |
| 52 | 0.43 | 0.37 | 0.07 | 0.31 | 0.79 | 0.44 | 0.57 | 0.53 | 0.59 | 0.00 | 0.00 |
| 53 | 0.03 | 0.03 | 0.00 | 0.00 | 0.15 | 0.01 | 0.03 | 0.03 | 0.04 | 0.00 | 0.00 |
| 54 | 0.38 | 0.33 | 0.03 | 0.20 | 0.66 | 0.38 | 0.50 | 0.55 | 0.62 | 0.00 | 0.00 |
| 55 | 0.03 | 0.03 | 0.00 | 0.00 | 0.15 | 0.01 | 0.03 | 0.03 | 0.05 | 0.00 | 0.00 |
| 56 | 0.34 | 0.29 | 0.02 | 0.14 | 0.64 | 0.31 | 0.44 | 0.51 | 0.59 | 0.00 | 0.00 |
| 57 | 0.02 | 0.01 | 0.00 | 0.00 | 0.07 | 0.00 | 0.02 | 0.02 | 0.01 | 0.00 | 0.00 |
| 58 | 0.22 | 0.18 | 0.01 | 0.05 | 0.42 | 0.16 | 0.32 | 0.38 | 0.24 | 0.00 | 0.00 |
| 59 | 0.00 | 0.00 | 0.00 | 0.00 | 0.01 | 0.00 | 0.01 | 0.01 | 0.00 | 0.00 | 0.00 |

TABLE S3. Posterior probability of existence of calcium isotopes according to all models.

| Z \ N | 30 | 31 | 32 | 33 | 34 | 35 | 36 | 37 | 38 | 39 | 40 | 41 | 42 | 43 | 44 | 45 | 46 | 47 | 48 | 49 | 50 | 51 | 52 | 53 | 54 | 55 | 56 | 57 | 58 | 59 |
|---|---|---|---|---|---|---|---|---|---|---|---|---|---|---|---|---|---|---|---|---|---|---|---|---|---|---|---|---|---|---|
| 14 | 1.00 | 0.91 | 1.00 | 0.31 | 0.97 | 0.00 | 0.04 | 0.00 | 0.01 | 0.00 | 0.00 | 0.00 | 0.00 | 0.00 | 0.00 | 0.00 | 0.00 | 0.00 | 0.00 | 0.00 | 0.00 | 0.00 | 0.00 | 0.00 | 0.00 | 0.00 | 0.00 | 0.00 | 0.00 | 0.00 |
| 15 | 1.00 | 1.00 | 1.00 | 0.74 | 1.00 | 0.00 | 0.31 | 0.00 | 0.09 | 0.00 | 0.02 | 0.00 | 0.00 | 0.00 | 0.00 | 0.00 | 0.00 | 0.00 | 0.00 | 0.00 | 0.00 | 0.00 | 0.00 | 0.00 | 0.00 | 0.00 | 0.00 | 0.00 | 0.00 | 0.00 |
| 16 | 1.00 | 1.00 | 1.00 | 0.90 | 1.00 | 0.10 | 0.75 | 0.05 | 0.53 | 0.01 | 0.22 | 0.00 | 0.01 | 0.00 | 0.01 | 0.00 | 0.02 | 0.00 | 0.00 | 0.00 | 0.00 | 0.00 | 0.00 | 0.00 | 0.00 | 0.00 | 0.00 | 0.00 | 0.00 | 0.00 |
| 17 | 1.00 | 1.00 | 1.00 | 1.00 | 1.00 | 0.66 | 1.00 | 0.32 | 0.97 | 0.05 | 0.73 | 0.00 | 0.05 | 0.00 | 0.03 | 0.00 | 0.04 | 0.00 | 0.01 | 0.00 | 0.01 | 0.00 | 0.00 | 0.00 | 0.00 | 0.00 | 0.00 | 0.00 | 0.00 | 0.00 |
| 18 | 1.00 | 1.00 | 1.00 | 1.00 | 1.00 | 0.88 | 1.00 | 0.86 | 1.00 | 0.35 | 0.96 | 0.01 | 0.37 | 0.01 | 0.21 | 0.01 | 0.27 | 0.00 | 0.14 | 0.00 | 0.13 | 0.00 | 0.09 | 0.00 | 0.03 | 0.00 | 0.01 | 0.00 | 0.02 | 0.00 |
| 19 | 1.00 | 1.00 | 1.00 | 1.00 | 1.00 | 1.00 | 1.00 | 0.99 | 1.00 | 0.82 | 1.00 | 0.11 | 0.90 | 0.02 | 0.60 | 0.02 | 0.54 | 0.01 | 0.40 | 0.00 | 0.28 | 0.00 | 0.24 | 0.00 | 0.12 | 0.00 | 0.07 | 0.00 | 0.06 | 0.00 |
| 20 | 1.00 | 1.00 | 1.00 | 1.00 | 1.00 | 1.00 | 1.00 | 1.00 | 1.00 | 0.98 | 1.00 | 0.55 | 0.99 | 0.19 | 0.88 | 0.09 | 0.76 | 0.08 | 0.72 | 0.04 | 0.60 | 0.04 | 0.57 | 0.03 | 0.50 | 0.03 | 0.44 | 0.02 | 0.32 | 0.01 |
| 21 | 1.00 | 1.00 | 1.00 | 1.00 | 1.00 | 1.00 | 1.00 | 1.00 | 1.00 | 1.00 | 1.00 | 0.95 | 1.00 | 0.62 | 1.00 | 0.57 | 1.00 | 0.32 | 0.98 | 0.14 | 0.90 | 0.08 | 0.80 | 0.06 | 0.73 | 0.05 | 0.67 | 0.03 | 0.51 | 0.01 |
| 22 | 1.00 | 1.00 | 1.00 | 1.00 | 1.00 | 1.00 | 1.00 | 1.00 | 1.00 | 1.00 | 1.00 | 0.99 | 1.00 | 0.92 | 1.00 | 0.95 | 1.00 | 0.72 | 1.00 | 0.40 | 0.96 | 0.23 | 0.88 | 0.19 | 0.84 | 0.18 | 0.80 | 0.14 | 0.69 | 0.06 |

TABLE S4. Posterior probability of existence of nuclei according to UNEDF0+GP. For the corresponding plot, see Fig. S6.

| Z \ N | 30 | 31 | 32 | 33 | 34 | 35 | 36 | 37 | 38 | 39 | 40 | 41 | 42 | 43 | 44 | 45 | 46 | 47 | 48 | 49 | 50 | 51 | 52 | 53 | 54 | 55 | 56 | 57 | 58 | 59 |
|---|---|---|---|---|---|---|---|---|---|---|---|---|---|---|---|---|---|---|---|---|---|---|---|---|---|---|---|---|---|---|
| 14 | 1.00 | 0.50 | 0.95 | 0.09 | 0.65 | 0.00 | 0.03 | 0.00 | 0.00 | 0.00 | 0.00 | 0.00 | 0.01 | 0.00 | 0.00 | 0.00 | 0.00 | 0.00 | 0.00 | 0.00 | 0.00 | 0.00 | 0.00 | 0.00 | 0.00 | 0.00 | 0.00 | 0.00 | 0.00 | 0.00 |
| 15 | 1.00 | 0.94 | 1.00 | 0.37 | 0.99 | 0.00 | 0.13 | 0.00 | 0.02 | 0.00 | 0.02 | 0.00 | 0.02 | 0.00 | 0.01 | 0.00 | 0.00 | 0.00 | 0.00 | 0.00 | 0.00 | 0.00 | 0.00 | 0.00 | 0.00 | 0.00 | 0.00 | 0.00 | 0.00 | 0.00 |
| 16 | 1.00 | 0.98 | 1.00 | 0.58 | 0.99 | 0.02 | 0.60 | 0.01 | 0.24 | 0.00 | 0.11 | 0.00 | 0.07 | 0.00 | 0.06 | 0.00 | 0.03 | 0.00 | 0.02 | 0.00 | 0.01 | 0.00 | 0.01 | 0.00 | 0.01 | 0.00 | 0.00 | 0.00 | 0.00 | 0.00 |
| 17 | 1.00 | 1.00 | 1.00 | 1.00 | 1.00 | 0.45 | 0.97 | 0.13 | 0.76 | 0.02 | 0.45 | 0.02 | 0.22 | 0.00 | 0.10 | 0.00 | 0.07 | 0.00 | 0.04 | 0.00 | 0.03 | 0.00 | 0.02 | 0.00 | 0.01 | 0.00 | 0.00 | 0.00 | 0.00 | 0.00 |
| 18 | 1.00 | 1.00 | 1.00 | 1.00 | 1.00 | 0.64 | 0.99 | 0.60 | 0.97 | 0.13 | 0.90 | 0.02 | 0.48 | 0.02 | 0.24 | 0.01 | 0.23 | 0.01 | 0.15 | 0.01 | 0.14 | 0.00 | 0.09 | 0.00 | 0.05 | 0.00 | 0.02 | 0.00 | 0.03 | 0.00 |
| 19 | 1.00 | 1.00 | 1.00 | 1.00 | 1.00 | 1.00 | 1.00 | 0.90 | 1.00 | 0.51 | 1.00 | 0.16 | 0.85 | 0.15 | 0.65 | 0.09 | 0.47 | 0.14 | 0.44 | 0.03 | 0.24 | 0.01 | 0.18 | 0.00 | 0.11 | 0.00 | 0.07 | 0.00 | 0.05 | 0.00 |
| 20 | 1.00 | 1.00 | 1.00 | 1.00 | 1.00 | 1.00 | 1.00 | 1.00 | 1.00 | 0.92 | 1.00 | 0.37 | 0.98 | 0.20 | 0.87 | 0.11 | 0.81 | 0.09 | 0.73 | 0.05 | 0.53 | 0.03 | 0.37 | 0.03 | 0.33 | 0.03 | 0.29 | 0.01 | 0.18 | 0.00 |
| 21 | 1.00 | 1.00 | 1.00 | 1.00 | 1.00 | 1.00 | 1.00 | 1.00 | 1.00 | 0.99 | 1.00 | 0.80 | 1.00 | 0.58 | 1.00 | 0.47 | 0.99 | 0.30 | 0.97 | 0.19 | 0.86 | 0.10 | 0.60 | 0.06 | 0.47 | 0.06 | 0.43 | 0.03 | 0.27 | 0.01 |
| 22 | 1.00 | 1.00 | 1.00 | 1.00 | 1.00 | 1.00 | 1.00 | 1.00 | 1.00 | 1.00 | 1.00 | 0.96 | 1.00 | 0.89 | 1.00 | 0.77 | 1.00 | 0.60 | 0.99 | 0.34 | 0.96 | 0.18 | 0.73 | 0.12 | 0.57 | 0.12 | 0.55 | 0.07 | 0.38 | 0.02 |

TABLE S5. Prior average of the posterior probabilities of existence of nuclei. For the corresponding plot, see Fig. 3.

| Z \ N | 30 | 31 | 32 | 33 | 34 | 35 | 36 | 37 | 38 | 39 | 40 | 41 | 42 | 43 | 44 | 45 | 46 | 47 | 48 | 49 | 50 | 51 | 52 | 53 | 54 | 55 | 56 | 57 | 58 | 59 |
|---|---|---|---|---|---|---|---|---|---|---|---|---|---|---|---|---|---|---|---|---|---|---|---|---|---|---|---|---|---|---|
| 14 | 1.00 | 0.60 | 0.94 | 0.14 | 0.73 | 0.00 | 0.03 | 0.00 | 0.01 | 0.00 | 0.01 | 0.00 | 0.01 | 0.00 | 0.00 | 0.00 | 0.00 | 0.00 | 0.00 | 0.00 | 0.00 | 0.00 | 0.00 | 0.00 | 0.00 | 0.00 | 0.00 | 0.00 | 0.00 | 0.00 |
| 15 | 1.00 | 0.96 | 1.00 | 0.46 | 0.99 | 0.00 | 0.18 | 0.00 | 0.04 | 0.00 | 0.02 | 0.00 | 0.02 | 0.00 | 0.01 | 0.00 | 0.00 | 0.00 | 0.00 | 0.00 | 0.00 | 0.00 | 0.00 | 0.00 | 0.00 | 0.00 | 0.00 | 0.00 | 0.00 | 0.00 |
| 16 | 1.00 | 0.99 | 1.00 | 0.69 | 1.00 | 0.04 | 0.66 | 0.02 | 0.32 | 0.00 | 0.14 | 0.01 | 0.08 | 0.00 | 0.06 | 0.00 | 0.03 | 0.00 | 0.02 | 0.00 | 0.01 | 0.00 | 0.01 | 0.00 | 0.01 | 0.00 | 0.00 | 0.00 | 0.00 | 0.00 |
| 17 | 1.00 | 1.00 | 1.00 | 1.00 | 1.00 | 0.53 | 0.98 | 0.20 | 0.85 | 0.02 | 0.55 | 0.01 | 0.18 | 0.00 | 0.11 | 0.00 | 0.08 | 0.00 | 0.05 | 0.00 | 0.04 | 0.00 | 0.02 | 0.00 | 0.01 | 0.00 | 0.00 | 0.00 | 0.00 | 0.00 |
| 18 | 1.00 | 1.00 | 1.00 | 1.00 | 1.00 | 0.69 | 0.99 | 0.71 | 0.98 | 0.18 | 0.92 | 0.02 | 0.49 | 0.02 | 0.24 | 0.02 | 0.26 | 0.01 | 0.17 | 0.01 | 0.16 | 0.01 | 0.10 | 0.00 | 0.05 | 0.00 | 0.02 | 0.00 | 0.03 | 0.00 |
| 19 | 1.00 | 1.00 | 1.00 | 1.00 | 1.00 | 1.00 | 1.00 | 0.94 | 1.00 | 0.60 | 1.00 | 0.20 | 0.88 | 0.11 | 0.67 | 0.07 | 0.53 | 0.08 | 0.43 | 0.02 | 0.27 | 0.01 | 0.21 | 0.00 | 0.12 | 0.00 | 0.08 | 0.00 | 0.06 | 0.00 |
| 20 | 1.00 | 1.00 | 1.00 | 1.00 | 1.00 | 1.00 | 1.00 | 1.00 | 1.00 | 0.94 | 1.00 | 0.46 | 0.98 | 0.21 | 0.88 | 0.13 | 0.82 | 0.10 | 0.76 | 0.06 | 0.57 | 0.04 | 0.43 | 0.03 | 0.38 | 0.03 | 0.34 | 0.02 | 0.22 | 0.00 |
| 21 | 1.00 | 1.00 | 1.00 | 1.00 | 1.00 | 1.00 | 1.00 | 1.00 | 1.00 | 1.00 | 1.00 | 0.87 | 1.00 | 0.64 | 1.00 | 0.55 | 1.00 | 0.37 | 0.98 | 0.22 | 0.89 | 0.09 | 0.63 | 0.06 | 0.54 | 0.07 | 0.50 | 0.03 | 0.33 | 0.01 |
| 22 | 1.00 | 1.00 | 1.00 | 1.00 | 1.00 | 1.00 | 1.00 | 1.00 | 1.00 | 1.00 | 1.00 | 0.98 | 1.00 | 0.92 | 1.00 | 0.86 | 1.00 | 0.66 | 1.00 | 0.39 | 0.96 | 0.19 | 0.73 | 0.14 | 0.63 | 0.14 | 0.61 | 0.09 | 0.47 | 0.03 |

TABLE S6. Posterior average of the posterior probabilities of existence of nuclei. For the corresponding plot, see Fig. 3.

| (Z, N) | posterior average | prior average | SLy4 | SkP | SkM* | SV-min | UNEDF0 | UNEDF1 | UNEDF2 | FRDM-2012 | HFB-24 |
|---|---|---|---|---|---|---|---|---|---|---|---|
| (14, 30) | 1.00 | 1.00 | 1.00 | 1.00 | 1.00 | 1.00 | 1.00 | 1.00 | 1.00 | 0.97 | 1.00 |
| (14, 31) | 0.60 | 0.50 | 0.12 | 0.45 | 0.89 | 0.60 | 0.91 | 0.70 | 0.72 | 0.00 | 0.11 |
| (14, 32) | 0.94 | 0.95 | 0.89 | 1.00 | 1.00 | 1.00 | 1.00 | 1.00 | 1.00 | 0.66 | 0.99 |
| (14, 33) | 0.14 | 0.09 | 0.01 | 0.01 | 0.19 | 0.07 | 0.31 | 0.22 | 0.02 | 0.00 | 0.01 |
| (14, 34) | 0.73 | 0.65 | 0.44 | 0.72 | 0.88 | 0.90 | 0.97 | 0.96 | 0.68 | 0.17 | 0.14 |
| (14, 35) | 0.00 | 0.00 | 0.00 | 0.00 | 0.00 | 0.00 | 0.00 | 0.00 | 0.00 | 0.00 | 0.03 |
| (14, 36) | 0.03 | 0.03 | 0.01 | 0.01 | 0.06 | 0.03 | 0.04 | 0.00 | 0.00 | 0.00 | 0.15 |
| (14, 37) | 0.00 | 0.00 | 0.00 | 0.00 | 0.00 | 0.00 | 0.00 | 0.00 | 0.00 | 0.00 | 0.00 |
| (14, 38) | 0.01 | 0.00 | 0.00 | 0.00 | 0.02 | 0.00 | 0.01 | 0.00 | 0.00 | 0.00 | 0.00 |
| (14, 39) | 0.00 | 0.00 | 0.00 | 0.00 | 0.00 | 0.00 | 0.00 | 0.00 | 0.00 | 0.00 | 0.00 |
| (14, 40) | 0.01 | 0.00 | 0.00 | 0.00 | 0.04 | 0.00 | 0.00 | 0.00 | 0.00 | 0.00 | 0.00 |
| (14, 41) | 0.00 | 0.00 | 0.00 | 0.00 | 0.00 | 0.00 | 0.00 | 0.00 | 0.00 | 0.00 | 0.00 |
| (14, 42) | 0.01 | 0.01 | 0.00 | 0.00 | 0.06 | 0.00 | 0.00 | 0.00 | 0.00 | 0.00 | 0.00 |
| (14, 43) | 0.00 | 0.00 | 0.00 | 0.00 | 0.00 | 0.00 | 0.00 | 0.00 | 0.00 | 0.00 | 0.00 |
| (14, 44) | 0.00 | 0.00 | 0.00 | 0.00 | 0.04 | 0.00 | 0.00 | 0.00 | 0.00 | 0.00 | 0.00 |
| (14, 45) | 0.00 | 0.00 | 0.00 | 0.00 | 0.00 | 0.00 | 0.00 | 0.00 | 0.00 | 0.00 | 0.00 |
| (14, 46) | 0.00 | 0.00 | 0.00 | 0.00 | 0.03 | 0.00 | 0.00 | 0.00 | 0.00 | 0.00 | 0.00 |
| (14, 47) | 0.00 | 0.00 | 0.00 | 0.00 | 0.00 | 0.00 | 0.00 | 0.00 | 0.00 | 0.00 | 0.00 |
| (14, 48) | 0.00 | 0.00 | 0.00 | 0.00 | 0.03 | 0.00 | 0.00 | 0.00 | 0.00 | 0.00 | 0.00 |
| (14, 49) | 0.00 | 0.00 | 0.00 | 0.00 | 0.00 | 0.00 | 0.00 | 0.00 | 0.00 | 0.00 | 0.00 |
| (14, 50) | 0.00 | 0.00 | 0.00 | 0.00 | 0.01 | 0.00 | 0.00 | 0.00 | 0.00 | 0.00 | 0.00 |
| (14, 51) | 0.00 | 0.00 | 0.00 | 0.00 | 0.00 | 0.00 | 0.00 | 0.00 | 0.00 | 0.00 | 0.00 |
| (14, 52) | 0.00 | 0.00 | 0.00 | 0.00 | 0.00 | 0.00 | 0.00 | 0.00 | 0.00 | 0.00 | 0.00 |
| (14, 53) | 0.00 | 0.00 | 0.00 | 0.00 | 0.00 | 0.00 | 0.00 | 0.00 | 0.00 | 0.00 | 0.00 |
| (14, 54) | 0.00 | 0.00 | 0.00 | 0.00 | 0.00 | 0.00 | 0.00 | 0.00 | 0.00 | 0.00 | 0.00 |
| (14, 55) | 0.00 | 0.00 | 0.00 | 0.00 | 0.00 | 0.00 | 0.00 | 0.00 | 0.00 | 0.00 | 0.00 |
| (14, 56) | 0.00 | 0.00 | 0.00 | 0.00 | 0.00 | 0.00 | 0.00 | 0.00 | 0.00 | 0.00 | 0.00 |
| (14, 57) | 0.00 | 0.00 | 0.00 | 0.00 | 0.00 | 0.00 | 0.00 | 0.00 | 0.00 | 0.00 | 0.00 |
| (14, 58) | 0.00 | 0.00 | 0.00 | 0.00 | 0.00 | 0.00 | 0.00 | 0.00 | 0.00 | 0.00 | 0.00 |
| (14, 59) | 0.00 | 0.00 | 0.00 | 0.00 | 0.00 | 0.00 | 0.00 | 0.00 | 0.00 | 0.00 | 0.00 |
| (15, 30) | 1.00 | 1.00 | 1.00 | 1.00 | 1.00 | 1.00 | 1.00 | 1.00 | 1.00 | 1.00 | 1.00 |
| (15, 31) | 0.96 | 0.94 | 0.85 | 0.97 | 1.00 | 0.99 | 1.00 | 1.00 | 0.99 | 0.92 | 0.71 |
| (15, 32) | 1.00 | 1.00 | 1.00 | 1.00 | 1.00 | 1.00 | 1.00 | 1.00 | 1.00 | 1.00 | 1.00 |
| (15, 33) | 0.46 | 0.37 | 0.20 | 0.20 | 0.57 | 0.45 | 0.74 | 0.64 | 0.24 | 0.11 | 0.17 |
| (15, 34) | 0.99 | 0.99 | 0.95 | 0.99 | 1.00 | 1.00 | 1.00 | 1.00 | 0.99 | 0.97 | 0.98 |
| (15, 35) | 0.00 | 0.00 | 0.00 | 0.00 | 0.00 | 0.00 | 0.00 | 0.00 | 0.00 | 0.00 | 0.00 |
| (15, 36) | 0.18 | 0.13 | 0.07 | 0.14 | 0.28 | 0.28 | 0.31 | 0.03 | 0.00 | 0.04 | 0.07 |
| (15, 37) | 0.00 | 0.00 | 0.00 | 0.00 | 0.00 | 0.00 | 0.00 | 0.00 | 0.00 | 0.00 | 0.00 |
| (15, 38) | 0.04 | 0.02 | 0.01 | 0.00 | 0.07 | 0.03 | 0.09 | 0.00 | 0.00 | 0.00 | 0.00 |
| (15, 39) | 0.00 | 0.00 | 0.00 | 0.00 | 0.00 | 0.00 | 0.00 | 0.00 | 0.00 | 0.00 | 0.00 |
| (15, 40) | 0.02 | 0.02 | 0.00 | 0.00 | 0.12 | 0.00 | 0.02 | 0.00 | 0.00 | 0.00 | 0.00 |
| (15, 41) | 0.00 | 0.00 | 0.00 | 0.00 | 0.00 | 0.00 | 0.00 | 0.00 | 0.00 | 0.00 | 0.00 |
| (15, 42) | 0.02 | 0.02 | 0.00 | 0.00 | 0.20 | 0.00 | 0.00 | 0.00 | 0.00 | 0.00 | 0.00 |
| (15, 43) | 0.00 | 0.00 | 0.00 | 0.00 | 0.00 | 0.00 | 0.00 | 0.00 | 0.00 | 0.00 | 0.00 |
| (15, 44) | 0.01 | 0.01 | 0.00 | 0.00 | 0.12 | 0.00 | 0.00 | 0.00 | 0.00 | 0.00 | 0.00 |
| (15, 45) | 0.00 | 0.00 | 0.00 | 0.00 | 0.00 | 0.00 | 0.00 | 0.00 | 0.00 | 0.00 | 0.00 |
| (15, 46) | 0.00 | 0.00 | 0.00 | 0.00 | 0.03 | 0.00 | 0.00 | 0.00 | 0.00 | 0.00 | 0.00 |
| (15, 47) | 0.00 | 0.00 | 0.00 | 0.00 | 0.00 | 0.00 | 0.00 | 0.00 | 0.00 | 0.00 | 0.00 |
| (15, 48) | 0.00 | 0.00 | 0.00 | 0.00 | 0.03 | 0.00 | 0.00 | 0.00 | 0.00 | 0.00 | 0.00 |
| (15, 49) | 0.00 | 0.00 | 0.00 | 0.00 | 0.00 | 0.00 | 0.00 | 0.00 | 0.00 | 0.00 | 0.00 |
| (15, 50) | 0.00 | 0.00 | 0.00 | 0.00 | 0.01 | 0.00 | 0.00 | 0.00 | 0.00 | 0.00 | 0.00 |
| (15, 51) | 0.00 | 0.00 | 0.00 | 0.00 | 0.00 | 0.00 | 0.00 | 0.00 | 0.00 | 0.00 | 0.00 |
| (15, 52) | 0.00 | 0.00 | 0.00 | 0.00 | 0.01 | 0.00 | 0.00 | 0.00 | 0.00 | 0.00 | 0.00 |
| (15, 53) | 0.00 | 0.00 | 0.00 | 0.00 | 0.00 | 0.00 | 0.00 | 0.00 | 0.00 | 0.00 | 0.00 |
| (15, 54) | 0.00 | 0.00 | 0.00 | 0.00 | 0.00 | 0.00 | 0.00 | 0.00 | 0.00 | 0.00 | 0.00 |
| (15, 55) | 0.00 | 0.00 | 0.00 | 0.00 | 0.00 | 0.00 | 0.00 | 0.00 | 0.00 | 0.00 | 0.00 |
| (15, 56) | 0.00 | 0.00 | 0.00 | 0.00 | 0.00 | 0.00 | 0.00 | 0.00 | 0.00 | 0.00 | 0.00 |
| (15, 57) | 0.00 | 0.00 | 0.00 | 0.00 | 0.00 | 0.00 | 0.00 | 0.00 | 0.00 | 0.00 | 0.00 |
| (15, 58) | 0.00 | 0.00 | 0.00 | 0.00 | 0.00 | 0.00 | 0.00 | 0.00 | 0.00 | 0.00 | 0.00 |
| (15, 59) | 0.00 | 0.00 | 0.00 | 0.00 | 0.00 | 0.00 | 0.00 | 0.00 | 0.00 | 0.00 | 0.00 |
| (16, 30) | 1.00 | 1.00 | 1.00 | 1.00 | 1.00 | 1.00 | 1.00 | 1.00 | 1.00 | 1.00 | 1.00 |
| (16, 31) | 0.99 | 0.98 | 0.87 | 1.00 | 1.00 | 1.00 | 1.00 | 1.00 | 1.00 | 1.00 | 0.96 |
| (16, 32) | 1.00 | 1.00 | 1.00 | 1.00 | 1.00 | 1.00 | 1.00 | 1.00 | 1.00 | 1.00 | 1.00 |
| (16, 33) | 0.69 | 0.58 | 0.33 | 0.49 | 0.72 | 0.68 | 0.90 | 0.83 | 0.29 | 0.65 | 0.35 |
| (16, 34) | 1.00 | 0.99 | 0.98 | 1.00 | 0.99 | 1.00 | 1.00 | 1.00 | 0.97 | 1.00 | 1.00 |
| (16, 35) | 0.04 | 0.02 | 0.01 | 0.00 | 0.05 | 0.03 | 0.10 | 0.01 | 0.00 | 0.00 | 0.00 |
| (16, 36) | 0.66 | 0.60 | 0.45 | 0.61 | 0.60 | 0.75 | 0.75 | 0.38 | 0.12 | 0.86 | 0.90 |
| (16, 37) | 0.02 | 0.01 | 0.00 | 0.00 | 0.02 | 0.00 | 0.05 | 0.00 | 0.00 | 0.00 | 0.00 |
| (16, 38) | 0.32 | 0.24 | 0.23 | 0.18 | 0.38 | 0.41 | 0.53 | 0.16 | 0.05 | 0.22 | 0.03 |
| (16, 39) | 0.00 | 0.00 | 0.00 | 0.00 | 0.02 | 0.00 | 0.01 | 0.00 | 0.00 | 0.00 | 0.00 |
| (16, 40) | 0.14 | 0.11 | 0.07 | 0.03 | 0.45 | 0.12 | 0.22 | 0.05 | 0.03 | 0.00 | 0.00 |
| (16, 41) | 0.01 | 0.00 | 0.00 | 0.00 | 0.04 | 0.00 | 0.00 | 0.00 | 0.00 | 0.00 | 0.00 |
| (16, 42) | 0.08 | 0.07 | 0.00 | 0.01 | 0.59 | 0.01 | 0.01 | 0.01 | 0.04 | 0.00 | 0.00 |
| (16, 43) | 0.00 | 0.00 | 0.00 | 0.00 | 0.02 | 0.00 | 0.00 | 0.00 | 0.00 | 0.00 | 0.00 |
| (16, 44) | 0.06 | 0.06 | 0.00 | 0.02 | 0.41 | 0.02 | 0.01 | 0.03 | 0.02 | 0.00 | 0.00 |
| (16, 45) | 0.00 | 0.00 | 0.00 | 0.00 | 0.01 | 0.00 | 0.00 | 0.00 | 0.00 | 0.00 | 0.00 |
| (16, 46) | 0.03 | 0.03 | 0.00 | 0.00 | 0.23 | 0.01 | 0.02 | 0.01 | 0.01 | 0.00 | 0.00 |
| (16, 47) | 0.00 | 0.00 | 0.00 | 0.00 | 0.00 | 0.00 | 0.00 | 0.00 | 0.00 | 0.00 | 0.00 |
| (16, 48) | 0.02 | 0.02 | 0.00 | 0.00 | 0.13 | 0.00 | 0.00 | 0.00 | 0.00 | 0.00 | 0.00 |
| (16, 49) | 0.00 | 0.00 | 0.00 | 0.00 | 0.00 | 0.00 | 0.00 | 0.00 | 0.00 | 0.00 | 0.00 |
| (16, 50) | 0.01 | 0.01 | 0.00 | 0.00 | 0.07 | 0.00 | 0.00 | 0.01 | 0.01 | 0.00 | 0.00 |
| (16, 51) | 0.00 | 0.00 | 0.00 | 0.00 | 0.00 | 0.00 | 0.00 | 0.00 | 0.00 | 0.00 | 0.00 |
| (16, 52) | 0.01 | 0.01 | 0.00 | 0.00 | 0.05 | 0.00 | 0.00 | 0.00 | 0.00 | 0.00 | 0.00 |
| (16, 53) | 0.00 | 0.00 | 0.00 | 0.00 | 0.00 | 0.00 | 0.00 | 0.00 | 0.00 | 0.00 | 0.00 |
| (16, 54) | 0.01 | 0.01 | 0.00 | 0.00 | 0.05 | 0.00 | 0.00 | 0.00 | 0.00 | 0.00 | 0.00 |
| (16, 55) | 0.00 | 0.00 | 0.00 | 0.00 | 0.00 | 0.00 | 0.00 | 0.00 | 0.00 | 0.00 | 0.00 |
| (16, 56) | 0.00 | 0.00 | 0.00 | 0.00 | 0.02 | 0.00 | 0.00 | 0.00 | 0.00 | 0.00 | 0.00 |
| (16, 57) | 0.00 | 0.00 | 0.00 | 0.00 | 0.00 | 0.00 | 0.00 | 0.00 | 0.00 | 0.00 | 0.00 |
| (16, 58) | 0.00 | 0.00 | 0.00 | 0.00 | 0.02 | 0.00 | 0.00 | 0.00 | 0.00 | 0.00 | 0.00 |
| (16, 59) | 0.00 | 0.00 | 0.00 | 0.00 | 0.00 | 0.00 | 0.00 | 0.00 | 0.00 | 0.00 | 0.00 |
| (17, 30) | 1.00 | 1.00 | 1.00 | 1.00 | 1.00 | 1.00 | 1.00 | 1.00 | 1.00 | 1.00 | 1.00 |
| (17, 31) | 1.00 | 1.00 | 1.00 | 1.00 | 1.00 | 1.00 | 1.00 | 1.00 | 1.00 | 1.00 | 1.00 |
| (17, 32) | 1.00 | 1.00 | 1.00 | 1.00 | 1.00 | 1.00 | 1.00 | 1.00 | 1.00 | 1.00 | 1.00 |
| (17, 33) | 1.00 | 1.00 | 1.00 | 1.00 | 1.00 | 1.00 | 1.00 | 1.00 | 1.00 | 1.00 | 1.00 |
| (17, 34) | 1.00 | 1.00 | 1.00 | 1.00 | 1.00 | 1.00 | 1.00 | 1.00 | 1.00 | 1.00 | 1.00 |
| (17, 35) | 0.53 | 0.45 | 0.39 | 0.33 | 0.46 | 0.54 | 0.66 | 0.32 | 0.14 | 0.81 | 0.41 |
| (17, 36) | 0.98 | 0.97 | 0.97 | 0.99 | 0.99 | 1.00 | 1.00 | 0.98 | 0.82 | 1.00 | 1.00 |
| (17, 37) | 0.20 | 0.13 | 0.08 | 0.02 | 0.11 | 0.14 | 0.32 | 0.07 | 0.02 | 0.42 | 0.03 |
| (17, 38) | 0.85 | 0.76 | 0.78 | 0.74 | 0.86 | 0.94 | 0.97 | 0.74 | 0.45 | 1.00 | 0.40 |
| (17, 39) | 0.02 | 0.02 | 0.01 | 0.00 | 0.06 | 0.02 | 0.05 | 0.01 | 0.01 | 0.01 | 0.00 |
| (17, 40) | 0.55 | 0.45 | 0.41 | 0.28 | 0.79 | 0.58 | 0.73 | 0.32 | 0.28 | 0.60 | 0.03 |
| (17, 41) | 0.01 | 0.02 | 0.00 | 0.00 | 0.06 | 0.00 | 0.00 | 0.00 | 0.00 | 0.00 | 0.11 |
| (17, 42) | 0.18 | 0.22 | 0.01 | 0.05 | 0.79 | 0.04 | 0.05 | 0.02 | 0.04 | 0.12 | 0.90 |
| (17, 43) | 0.00 | 0.00 | 0.00 | 0.00 | 0.04 | 0.00 | 0.00 | 0.00 | 0.00 | 0.00 | 0.00 |
| (17, 44) | 0.11 | 0.10 | 0.00 | 0.03 | 0.72 | 0.03 | 0.03 | 0.04 | 0.05 | 0.00 | 0.03 |
| (17, 45) | 0.00 | 0.00 | 0.00 | 0.00 | 0.02 | 0.00 | 0.00 | 0.00 | 0.00 | 0.00 | 0.01 |
| (17, 46) | 0.08 | 0.07 | 0.01 | 0.01 | 0.54 | 0.04 | 0.04 | 0.02 | 0.02 | 0.00 | 0.00 |
| (17, 47) | 0.00 | 0.00 | 0.00 | 0.00 | 0.01 | 0.00 | 0.00 | 0.00 | 0.00 | 0.00 | 0.01 |
| (17, 48) | 0.05 | 0.04 | 0.00 | 0.00 | 0.34 | 0.01 | 0.01 | 0.01 | 0.01 | 0.00 | 0.00 |
| (17, 49) | 0.00 | 0.00 | 0.00 | 0.00 | 0.00 | 0.00 | 0.00 | 0.00 | 0.00 | 0.00 | 0.00 |
| (17, 50) | 0.04 | 0.03 | 0.00 | 0.00 | 0.25 | 0.00 | 0.01 | 0.02 | 0.01 | 0.00 | 0.00 |
| (17, 51) | 0.00 | 0.00 | 0.00 | 0.00 | 0.00 | 0.00 | 0.00 | 0.00 | 0.00 | 0.00 | 0.00 |
| (17, 52) | 0.02 | 0.02 | 0.00 | 0.00 | 0.18 | 0.00 | 0.00 | 0.01 | 0.00 | 0.00 | 0.00 |
| (17, 53) | 0.00 | 0.00 | 0.00 | 0.00 | 0.00 | 0.00 | 0.00 | 0.00 | 0.00 | 0.00 | 0.00 |
| (17, 54) | 0.01 | 0.01 | 0.00 | 0.00 | 0.09 | 0.00 | 0.00 | 0.00 | 0.00 | 0.00 | 0.00 |
| (17, 55) | 0.00 | 0.00 | 0.00 | 0.00 | 0.00 | 0.00 | 0.00 | 0.00 | 0.00 | 0.00 | 0.00 |
| (17, 56) | 0.00 | 0.00 | 0.00 | 0.00 | 0.03 | 0.00 | 0.00 | 0.00 | 0.00 | 0.00 | 0.00 |
| (17, 57) | 0.00 | 0.00 | 0.00 | 0.00 | 0.00 | 0.00 | 0.00 | 0.00 | 0.00 | 0.00 | 0.00 |
| (17, 58) | 0.00 | 0.00 | 0.00 | 0.00 | 0.04 | 0.00 | 0.00 | 0.00 | 0.00 | 0.00 | 0.00 |
| (17, 59) | 0.00 | 0.00 | 0.00 | 0.00 | 0.00 | 0.00 | 0.00 | 0.00 | 0.00 | 0.00 | 0.00 |
| (18, 30) | 1.00 | 1.00 | 1.00 | 1.00 | 1.00 | 1.00 | 1.00 | 1.00 | 1.00 | 1.00 | 1.00 |
| (18, 31) | 1.00 | 1.00 | 1.00 | 1.00 | 1.00 | 1.00 | 1.00 | 1.00 | 1.00 | 1.00 | 1.00 |
| (18, 32) | 1.00 | 1.00 | 1.00 | 1.00 | 1.00 | 1.00 | 1.00 | 1.00 | 1.00 | 1.00 | 1.00 |
| (18, 33) | 1.00 | 1.00 | 1.00 | 1.00 | 1.00 | 1.00 | 1.00 | 1.00 | 0.99 | 1.00 | 1.00 |
| (18, 34) | 1.00 | 1.00 | 1.00 | 1.00 | 1.00 | 1.00 | 1.00 | 1.00 | 1.00 | 1.00 | 1.00 |
| (18, 35) | 0.69 | 0.64 | 0.58 | 0.64 | 0.68 | 0.78 | 0.88 | 0.71 | 0.38 | 0.50 | 0.59 |
| (18, 36) | 0.99 | 0.99 | 0.99 | 1.00 | 0.98 | 1.00 | 1.00 | 1.00 | 0.95 | 1.00 | 1.00 |
| (18, 37) | 0.71 | 0.60 | 0.53 | 0.41 | 0.66 | 0.68 | 0.86 | 0.62 | 0.42 | 0.94 | 0.30 |
| (18, 38) | 0.98 | 0.97 | 0.97 | 0.97 | 0.96 | 0.99 | 1.00 | 0.97 | 0.91 | 1.00 | 1.00 |
| (18, 39) | 0.18 | 0.13 | 0.09 | 0.03 | 0.32 | 0.13 | 0.35 | 0.10 | 0.06 | 0.09 | 0.00 |
| (18, 40) | 0.92 | 0.90 | 0.86 | 0.79 | 0.94 | 0.93 | 0.96 | 0.81 | 0.80 | 1.00 | 0.99 |
| (18, 41) | 0.02 | 0.02 | 0.00 | 0.00 | 0.18 | 0.00 | 0.01 | 0.00 | 0.00 | 0.00 | 0.00 |
| (18, 42) | 0.49 | 0.48 | 0.20 | 0.42 | 0.88 | 0.38 | 0.37 | 0.17 | 0.15 | 0.83 | 0.93 |
| (18, 43) | 0.02 | 0.02 | 0.00 | 0.00 | 0.18 | 0.00 | 0.01 | 0.00 | 0.00 | 0.00 | 0.00 |
| (18, 44) | 0.24 | 0.24 | 0.03 | 0.16 | 0.88 | 0.15 | 0.21 | 0.20 | 0.22 | 0.00 | 0.33 |
| (18, 45) | 0.02 | 0.01 | 0.00 | 0.00 | 0.12 | 0.00 | 0.01 | 0.00 | 0.00 | 0.00 | 0.00 |
| (18, 46) | 0.26 | 0.23 | 0.10 | 0.16 | 0.80 | 0.24 | 0.27 | 0.20 | 0.21 | 0.02 | 0.05 |
| (18, 47) | 0.01 | 0.01 | 0.00 | 0.00 | 0.09 | 0.00 | 0.00 | 0.00 | 0.00 | 0.00 | 0.00 |
| (18, 48) | 0.17 | 0.15 | 0.02 | 0.07 | 0.71 | 0.12 | 0.14 | 0.15 | 0.16 | 0.00 | 0.00 |
| (18, 49) | 0.01 | 0.01 | 0.00 | 0.00 | 0.06 | 0.00 | 0.00 | 0.00 | 0.00 | 0.00 | 0.00 |
| (18, 50) | 0.16 | 0.14 | 0.01 | 0.05 | 0.63 | 0.09 | 0.13 | 0.17 | 0.17 | 0.00 | 0.00 |
| (18, 51) | 0.01 | 0.00 | 0.00 | 0.00 | 0.04 | 0.00 | 0.00 | 0.00 | 0.00 | 0.00 | 0.00 |
| (18, 52) | 0.10 | 0.09 | 0.01 | 0.02 | 0.47 | 0.07 | 0.09 | 0.08 | 0.08 | 0.00 | 0.00 |
| (18, 53) | 0.00 | 0.00 | 0.00 | 0.00 | 0.02 | 0.00 | 0.00 | 0.00 | 0.00 | 0.00 | 0.00 |
| (18, 54) | 0.05 | 0.05 | 0.00 | 0.00 | 0.29 | 0.02 | 0.03 | 0.03 | 0.02 | 0.00 | 0.00 |
| (18, 55) | 0.00 | 0.00 | 0.00 | 0.00 | 0.00 | 0.00 | 0.00 | 0.00 | 0.00 | 0.00 | 0.00 |
| (18, 56) | 0.02 | 0.02 | 0.00 | 0.00 | 0.12 | 0.00 | 0.01 | 0.01 | 0.01 | 0.00 | 0.00 |
| (18, 57) | 0.00 | 0.00 | 0.00 | 0.00 | 0.01 | 0.00 | 0.00 | 0.00 | 0.00 | 0.00 | 0.00 |
| (18, 58) | 0.03 | 0.03 | 0.00 | 0.00 | 0.19 | 0.01 | 0.02 | 0.01 | 0.04 | 0.00 | 0.00 |
| (18, 59) | 0.00 | 0.00 | 0.00 | 0.00 | 0.00 | 0.00 | 0.00 | 0.00 | 0.00 | 0.00 | 0.00 |
| (19, 30) | 1.00 | 1.00 | 1.00 | 1.00 | 1.00 | 1.00 | 1.00 | 1.00 | 1.00 | 1.00 | 1.00 |
| (19, 31) | 1.00 | 1.00 | 1.00 | 1.00 | 1.00 | 1.00 | 1.00 | 1.00 | 1.00 | 1.00 | 1.00 |
| (19, 32) | 1.00 | 1.00 | 1.00 | 1.00 | 1.00 | 1.00 | 1.00 | 1.00 | 1.00 | 1.00 | 1.00 |
| (19, 33) | 1.00 | 1.00 | 1.00 | 1.00 | 1.00 | 1.00 | 1.00 | 1.00 | 1.00 | 1.00 | 1.00 |
| (19, 34) | 1.00 | 1.00 | 1.00 | 1.00 | 1.00 | 1.00 | 1.00 | 1.00 | 1.00 | 1.00 | 1.00 |
| (19, 35) | 1.00 | 1.00 | 1.00 | 1.00 | 1.00 | 1.00 | 1.00 | 1.00 | 1.00 | 1.00 | 1.00 |
| (19, 36) | 1.00 | 1.00 | 1.00 | 1.00 | 1.00 | 1.00 | 1.00 | 1.00 | 1.00 | 1.00 | 1.00 |
| (19, 37) | 0.94 | 0.90 | 0.88 | 0.83 | 0.92 | 0.96 | 0.99 | 0.95 | 0.80 | 1.00 | 0.78 |
| (19, 38) | 1.00 | 1.00 | 1.00 | 1.00 | 1.00 | 1.00 | 1.00 | 1.00 | 1.00 | 1.00 | 1.00 |
| (19, 39) | 0.60 | 0.51 | 0.42 | 0.34 | 0.71 | 0.58 | 0.82 | 0.53 | 0.41 | 0.49 | 0.34 |
| (19, 40) | 1.00 | 1.00 | 1.00 | 1.00 | 1.00 | 1.00 | 1.00 | 1.00 | 1.00 | 1.00 | 1.00 |
| (19, 41) | 0.20 | 0.16 | 0.04 | 0.05 | 0.51 | 0.07 | 0.11 | 0.03 | 0.02 | 0.57 | 0.00 |
| (19, 42) | 0.88 | 0.85 | 0.67 | 0.91 | 1.00 | 0.89 | 0.90 | 0.66 | 0.62 | 1.00 | 0.99 |
| (19, 43) | 0.11 | 0.15 | 0.00 | 0.01 | 0.45 | 0.02 | 0.02 | 0.01 | 0.01 | 0.10 | 0.73 |
| (19, 44) | 0.67 | 0.65 | 0.22 | 0.60 | 0.99 | 0.55 | 0.60 | 0.44 | 0.46 | 0.97 | 0.99 |
| (19, 45) | 0.07 | 0.09 | 0.01 | 0.00 | 0.34 | 0.01 | 0.02 | 0.01 | 0.02 | 0.00 | 0.40 |
| (19, 46) | 0.53 | 0.47 | 0.27 | 0.44 | 0.98 | 0.52 | 0.54 | 0.40 | 0.50 | 0.56 | 0.00 |
| (19, 47) | 0.08 | 0.14 | 0.00 | 0.00 | 0.23 | 0.01 | 0.01 | 0.01 | 0.01 | 0.00 | 1.00 |
| (19, 48) | 0.43 | 0.44 | 0.12 | 0.20 | 0.95 | 0.31 | 0.40 | 0.33 | 0.35 | 0.31 | 1.00 |
| (19, 49) | 0.02 | 0.03 | 0.00 | 0.00 | 0.13 | 0.00 | 0.00 | 0.01 | 0.01 | 0.00 | 0.13 |
| (19, 50) | 0.27 | 0.24 | 0.03 | 0.13 | 0.88 | 0.19 | 0.28 | 0.30 | 0.32 | 0.01 | 0.00 |
| (19, 51) | 0.01 | 0.01 | 0.00 | 0.00 | 0.06 | 0.00 | 0.00 | 0.00 | 0.01 | 0.00 | 0.00 |
| (19, 52) | 0.21 | 0.18 | 0.01 | 0.06 | 0.68 | 0.15 | 0.24 | 0.21 | 0.23 | 0.00 | 0.00 |
| (19, 53) | 0.00 | 0.00 | 0.00 | 0.00 | 0.03 | 0.00 | 0.00 | 0.00 | 0.00 | 0.00 | 0.00 |
| (19, 54) | 0.12 | 0.11 | 0.00 | 0.02 | 0.47 | 0.08 | 0.12 | 0.13 | 0.15 | 0.00 | 0.00 |
| (19, 55) | 0.00 | 0.00 | 0.00 | 0.00 | 0.02 | 0.00 | 0.00 | 0.00 | 0.00 | 0.00 | 0.00 |
| (19, 56) | 0.08 | 0.07 | 0.00 | 0.01 | 0.31 | 0.03 | 0.07 | 0.08 | 0.11 | 0.00 | 0.00 |
| (19, 57) | 0.00 | 0.00 | 0.00 | 0.00 | 0.01 | 0.00 | 0.00 | 0.00 | 0.00 | 0.00 | 0.00 |
| (19, 58) | 0.06 | 0.05 | 0.00 | 0.00 | 0.25 | 0.03 | 0.06 | 0.05 | 0.08 | 0.00 | 0.00 |
| (19, 59) | 0.00 | 0.00 | 0.00 | 0.00 | 0.00 | 0.00 | 0.00 | 0.00 | 0.00 | 0.00 | 0.00 |
| (20, 30) | 1.00 | 1.00 | 1.00 | 1.00 | 1.00 | 1.00 | 1.00 | 1.00 | 1.00 | 1.00 | 1.00 |
| (20, 31) | 1.00 | 1.00 | 1.00 | 1.00 | 1.00 | 1.00 | 1.00 | 1.00 | 1.00 | 1.00 | 1.00 |
| (20, 32) | 1.00 | 1.00 | 1.00 | 1.00 | 1.00 | 1.00 | 1.00 | 1.00 | 1.00 | 1.00 | 1.00 |
| (20, 33) | 1.00 | 1.00 | 1.00 | 1.00 | 1.00 | 1.00 | 1.00 | 1.00 | 1.00 | 1.00 | 1.00 |
| (20, 34) | 1.00 | 1.00 | 1.00 | 1.00 | 1.00 | 1.00 | 1.00 | 1.00 | 1.00 | 1.00 | 1.00 |
| (20, 35) | 1.00 | 1.00 | 1.00 | 1.00 | 1.00 | 1.00 | 1.00 | 1.00 | 1.00 | 1.00 | 1.00 |
| (20, 36) | 1.00 | 1.00 | 1.00 | 1.00 | 1.00 | 1.00 | 1.00 | 1.00 | 1.00 | 1.00 | 1.00 |
| (20, 37) | 1.00 | 1.00 | 1.00 | 1.00 | 1.00 | 1.00 | 1.00 | 1.00 | 1.00 | 1.00 | 1.00 |
| (20, 38) | 1.00 | 1.00 | 1.00 | 1.00 | 1.00 | 1.00 | 1.00 | 1.00 | 1.00 | 1.00 | 1.00 |
| (20, 39) | 0.94 | 0.92 | 0.81 | 0.84 | 0.95 | 0.93 | 0.98 | 0.93 | 0.86 | 1.00 | 0.98 |
| (20, 40) | 1.00 | 1.00 | 1.00 | 1.00 | 1.00 | 1.00 | 1.00 | 1.00 | 1.00 | 1.00 | 1.00 |
| (20, 41) | 0.46 | 0.37 | 0.18 | 0.30 | 0.84 | 0.36 | 0.55 | 0.25 | 0.16 | 0.56 | 0.15 |
| (20, 42) | 0.98 | 0.98 | 0.94 | 0.99 | 1.00 | 0.99 | 0.99 | 0.95 | 0.93 | 1.00 | 1.00 |
| (20, 43) | 0.21 | 0.20 | 0.04 | 0.06 | 0.74 | 0.09 | 0.19 | 0.06 | 0.04 | 0.16 | 0.47 |
| (20, 44) | 0.88 | 0.87 | 0.69 | 0.92 | 1.00 | 0.87 | 0.88 | 0.72 | 0.71 | 1.00 | 1.00 |
| (20, 45) | 0.13 | 0.11 | 0.03 | 0.01 | 0.66 | 0.04 | 0.09 | 0.04 | 0.04 | 0.07 | 0.00 |
| (20, 46) | 0.82 | 0.81 | 0.62 | 0.76 | 0.99 | 0.77 | 0.76 | 0.63 | 0.75 | 1.00 | 0.99 |
| (20, 47) | 0.10 | 0.09 | 0.02 | 0.00 | 0.58 | 0.02 | 0.08 | 0.03 | 0.03 | 0.03 | 0.00 |
| (20, 48) | 0.76 | 0.73 | 0.51 | 0.58 | 0.99 | 0.64 | 0.72 | 0.62 | 0.69 | 0.96 | 0.92 |
| (20, 49) | 0.06 | 0.05 | 0.00 | 0.00 | 0.35 | 0.01 | 0.04 | 0.02 | 0.02 | 0.00 | 0.00 |
| (20, 50) | 0.57 | 0.53 | 0.25 | 0.42 | 0.94 | 0.49 | 0.60 | 0.55 | 0.61 | 0.48 | 0.39 |
| (20, 51) | 0.04 | 0.03 | 0.00 | 0.00 | 0.20 | 0.01 | 0.04 | 0.03 | 0.03 | 0.00 | 0.00 |
| (20, 52) | 0.43 | 0.37 | 0.07 | 0.31 | 0.79 | 0.44 | 0.57 | 0.53 | 0.59 | 0.00 | 0.00 |
| (20, 53) | 0.03 | 0.03 | 0.00 | 0.00 | 0.15 | 0.01 | 0.03 | 0.03 | 0.04 | 0.00 | 0.00 |
| (20, 54) | 0.38 | 0.33 | 0.03 | 0.20 | 0.66 | 0.38 | 0.50 | 0.55 | 0.62 | 0.00 | 0.00 |
| (20, 55) | 0.03 | 0.03 | 0.00 | 0.00 | 0.15 | 0.01 | 0.03 | 0.03 | 0.05 | 0.00 | 0.00 |
| (20, 56) | 0.34 | 0.29 | 0.02 | 0.14 | 0.64 | 0.31 | 0.44 | 0.51 | 0.59 | 0.00 | 0.00 |
| (20, 57) | 0.02 | 0.01 | 0.00 | 0.00 | 0.07 | 0.00 | 0.02 | 0.02 | 0.01 | 0.00 | 0.00 |
| (20, 58) | 0.22 | 0.18 | 0.01 | 0.05 | 0.42 | 0.16 | 0.32 | 0.38 | 0.24 | 0.00 | 0.00 |
| (20, 59) | 0.00 | 0.00 | 0.00 | 0.00 | 0.01 | 0.00 | 0.01 | 0.01 | 0.00 | 0.00 | 0.00 |
| (21, 30) | 1.00 | 1.00 | 1.00 | 1.00 | 1.00 | 1.00 | 1.00 | 1.00 | 1.00 | 1.00 | 1.00 |
| (21, 31) | 1.00 | 1.00 | 1.00 | 1.00 | 1.00 | 1.00 | 1.00 | 1.00 | 1.00 | 1.00 | 1.00 |
| (21, 32) | 1.00 | 1.00 | 1.00 | 1.00 | 1.00 | 1.00 | 1.00 | 1.00 | 1.00 | 1.00 | 1.00 |
| (21, 33) | 1.00 | 1.00 | 1.00 | 1.00 | 1.00 | 1.00 | 1.00 | 1.00 | 1.00 | 1.00 | 1.00 |
| (21, 34) | 1.00 | 1.00 | 1.00 | 1.00 | 1.00 | 1.00 | 1.00 | 1.00 | 1.00 | 1.00 | 1.00 |
| (21, 35) | 1.00 | 1.00 | 1.00 | 1.00 | 1.00 | 1.00 | 1.00 | 1.00 | 1.00 | 1.00 | 1.00 |
| (21, 36) | 1.00 | 1.00 | 1.00 | 1.00 | 1.00 | 1.00 | 1.00 | 1.00 | 1.00 | 1.00 | 1.00 |
| (21, 37) | 1.00 | 1.00 | 1.00 | 1.00 | 1.00 | 1.00 | 1.00 | 1.00 | 1.00 | 1.00 | 1.00 |
| (21, 38) | 1.00 | 1.00 | 1.00 | 1.00 | 1.00 | 1.00 | 1.00 | 1.00 | 1.00 | 1.00 | 1.00 |
| (21, 39) | 1.00 | 0.99 | 0.98 | 0.98 | 1.00 | 1.00 | 1.00 | 1.00 | 0.99 | 1.00 | 1.00 |
| (21, 40) | 1.00 | 1.00 | 1.00 | 1.00 | 1.00 | 1.00 | 1.00 | 1.00 | 1.00 | 1.00 | 1.00 |
| (21, 41) | 0.87 | 0.80 | 0.63 | 0.80 | 0.98 | 0.84 | 0.95 | 0.79 | 0.63 | 1.00 | 0.59 |
| (21, 42) | 1.00 | 1.00 | 1.00 | 1.00 | 1.00 | 1.00 | 1.00 | 1.00 | 1.00 | 1.00 | 1.00 |
| (21, 43) | 0.64 | 0.58 | 0.29 | 0.41 | 0.96 | 0.47 | 0.62 | 0.51 | 0.49 | 0.99 | 0.45 |
| (21, 44) | 1.00 | 1.00 | 0.98 | 1.00 | 1.00 | 1.00 | 1.00 | 1.00 | 1.00 | 1.00 | 1.00 |
| (21, 45) | 0.55 | 0.47 | 0.21 | 0.23 | 0.95 | 0.37 | 0.57 | 0.36 | 0.35 | 0.90 | 0.28 |
| (21, 46) | 1.00 | 0.99 | 0.96 | 0.99 | 1.00 | 1.00 | 1.00 | 0.99 | 0.99 | 1.00 | 1.00 |
| (21, 47) | 0.37 | 0.30 | 0.16 | 0.09 | 0.86 | 0.17 | 0.32 | 0.20 | 0.18 | 0.69 | 0.06 |
| (21, 48) | 0.98 | 0.97 | 0.92 | 0.96 | 1.00 | 0.97 | 0.98 | 0.95 | 0.95 | 1.00 | 1.00 |
| (21, 49) | 0.22 | 0.19 | 0.05 | 0.03 | 0.66 | 0.08 | 0.14 | 0.09 | 0.09 | 0.51 | 0.02 |
| (21, 50) | 0.89 | 0.86 | 0.64 | 0.80 | 1.00 | 0.85 | 0.90 | 0.83 | 0.86 | 1.00 | 0.90 |
| (21, 51) | 0.09 | 0.10 | 0.01 | 0.01 | 0.30 | 0.04 | 0.08 | 0.06 | 0.09 | 0.00 | 0.27 |
| (21, 52) | 0.63 | 0.60 | 0.13 | 0.60 | 0.94 | 0.70 | 0.80 | 0.74 | 0.83 | 0.00 | 0.64 |
| (21, 53) | 0.06 | 0.06 | 0.00 | 0.01 | 0.22 | 0.03 | 0.06 | 0.07 | 0.09 | 0.00 | 0.04 |
| (21, 54) | 0.54 | 0.47 | 0.03 | 0.42 | 0.83 | 0.57 | 0.73 | 0.76 | 0.76 | 0.00 | 0.12 |
| (21, 55) | 0.07 | 0.06 | 0.00 | 0.00 | 0.24 | 0.04 | 0.05 | 0.07 | 0.13 | 0.00 | 0.01 |
| (21, 56) | 0.50 | 0.43 | 0.03 | 0.29 | 0.81 | 0.52 | 0.67 | 0.71 | 0.80 | 0.00 | 0.04 |
| (21, 57) | 0.03 | 0.03 | 0.00 | 0.00 | 0.09 | 0.02 | 0.03 | 0.05 | 0.03 | 0.00 | 0.00 |
| (21, 58) | 0.33 | 0.27 | 0.01 | 0.07 | 0.57 | 0.26 | 0.51 | 0.59 | 0.39 | 0.00 | 0.00 |
| (21, 59) | 0.01 | 0.01 | 0.00 | 0.00 | 0.01 | 0.00 | 0.01 | 0.02 | 0.00 | 0.00 | 0.01 |
| (22, 30) | 1.00 | 1.00 | 1.00 | 1.00 | 1.00 | 1.00 | 1.00 | 1.00 | 1.00 | 1.00 | 1.00 |
| (22, 31) | 1.00 | 1.00 | 1.00 | 1.00 | 1.00 | 1.00 | 1.00 | 1.00 | 1.00 | 1.00 | 1.00 |
| (22, 32) | 1.00 | 1.00 | 1.00 | 1.00 | 1.00 | 1.00 | 1.00 | 1.00 | 1.00 | 1.00 | 1.00 |
| (22, 33) | 1.00 | 1.00 | 1.00 | 1.00 | 1.00 | 1.00 | 1.00 | 1.00 | 1.00 | 1.00 | 1.00 |
| (22, 34) | 1.00 | 1.00 | 1.00 | 1.00 | 1.00 | 1.00 | 1.00 | 1.00 | 1.00 | 1.00 | 1.00 |
| (22, 35) | 1.00 | 1.00 | 1.00 | 1.00 | 1.00 | 1.00 | 1.00 | 1.00 | 1.00 | 1.00 | 1.00 |
| (22, 36) | 1.00 | 1.00 | 1.00 | 1.00 | 1.00 | 1.00 | 1.00 | 1.00 | 1.00 | 1.00 | 1.00 |
| (22, 37) | 1.00 | 1.00 | 1.00 | 1.00 | 1.00 | 1.00 | 1.00 | 1.00 | 1.00 | 1.00 | 1.00 |
| (22, 38) | 1.00 | 1.00 | 1.00 | 1.00 | 1.00 | 1.00 | 1.00 | 1.00 | 1.00 | 1.00 | 1.00 |
| (22, 39) | 1.00 | 1.00 | 1.00 | 1.00 | 1.00 | 1.00 | 1.00 | 1.00 | 1.00 | 1.00 | 1.00 |
| (22, 40) | 1.00 | 1.00 | 1.00 | 1.00 | 1.00 | 1.00 | 1.00 | 1.00 | 1.00 | 1.00 | 1.00 |
| (22, 41) | 0.98 | 0.96 | 0.89 | 0.98 | 0.99 | 0.98 | 0.99 | 0.98 | 0.91 | 1.00 | 0.89 |
| (22, 42) | 1.00 | 1.00 | 1.00 | 1.00 | 1.00 | 1.00 | 1.00 | 1.00 | 1.00 | 1.00 | 1.00 |
| (22, 43) | 0.92 | 0.89 | 0.63 | 0.83 | 0.99 | 0.88 | 0.92 | 0.94 | 0.95 | 0.98 | 0.93 |
| (22, 44) | 1.00 | 1.00 | 1.00 | 1.00 | 1.00 | 1.00 | 1.00 | 1.00 | 1.00 | 1.00 | 1.00 |
| (22, 45) | 0.86 | 0.77 | 0.55 | 0.70 | 0.99 | 0.86 | 0.95 | 0.88 | 0.80 | 0.89 | 0.34 |
| (22, 46) | 1.00 | 1.00 | 0.99 | 1.00 | 1.00 | 1.00 | 1.00 | 1.00 | 1.00 | 1.00 | 1.00 |
| (22, 47) | 0.66 | 0.60 | 0.49 | 0.38 | 0.95 | 0.55 | 0.72 | 0.56 | 0.45 | 0.78 | 0.53 |
| (22, 48) | 1.00 | 0.99 | 0.99 | 0.99 | 1.00 | 1.00 | 1.00 | 0.99 | 0.99 | 1.00 | 1.00 |
| (22, 49) | 0.39 | 0.34 | 0.18 | 0.12 | 0.85 | 0.23 | 0.40 | 0.28 | 0.24 | 0.51 | 0.19 |
| (22, 50) | 0.96 | 0.96 | 0.90 | 0.94 | 1.00 | 0.95 | 0.96 | 0.92 | 0.94 | 1.00 | 1.00 |
| (22, 51) | 0.19 | 0.18 | 0.02 | 0.04 | 0.52 | 0.11 | 0.23 | 0.17 | 0.22 | 0.00 | 0.30 |
| (22, 52) | 0.73 | 0.73 | 0.35 | 0.81 | 0.95 | 0.84 | 0.88 | 0.83 | 0.91 | 0.06 | 0.96 |
| (22, 53) | 0.14 | 0.12 | 0.01 | 0.02 | 0.40 | 0.06 | 0.19 | 0.20 | 0.15 | 0.00 | 0.01 |
| (22, 54) | 0.63 | 0.57 | 0.15 | 0.67 | 0.86 | 0.72 | 0.84 | 0.85 | 0.80 | 0.00 | 0.23 |
| (22, 55) | 0.14 | 0.12 | 0.01 | 0.01 | 0.41 | 0.08 | 0.18 | 0.17 | 0.25 | 0.00 | 0.01 |
| (22, 56) | 0.61 | 0.55 | 0.14 | 0.55 | 0.86 | 0.71 | 0.80 | 0.79 | 0.86 | 0.00 | 0.21 |
| (22, 57) | 0.09 | 0.07 | 0.00 | 0.00 | 0.20 | 0.03 | 0.14 | 0.16 | 0.07 | 0.00 | 0.00 |
| (22, 58) | 0.47 | 0.38 | 0.06 | 0.24 | 0.67 | 0.47 | 0.69 | 0.75 | 0.58 | 0.00 | 0.00 |
| (22, 59) | 0.03 | 0.02 | 0.00 | 0.00 | 0.04 | 0.00 | 0.06 | 0.04 | 0.00 | 0.00 | 0.00 |

TABLE S7. Posterior probability of existence of nuclei $p_{ex}$ according to various nuclear models.
